# Supplementary material for: GLIME: General, Stable and Local LIME Explanation
Source: arXiv:2311.15722 source file (2023-11-27)
Supplement: Supplementary file 1 [file proof_new.tex]

\section{Proofs}
In this section, we provide the detailed proofs of theoretical results presented in the main part. 

Before diving into proofs, we first derive ${\*w}_n^{\text{GeneralLIME}}$ and its limit $\*w$ since they will be used across all proofs. 

\subsection{Expression of ${\*w}_n^{\text{GeneralLIME}}$ and $\*w$}
\begin{proposition}
When sample size $n\to\infty$, the explanation ${\*w}_n^{\text{LIME}}$ returned by LIME and the explanation ${\*w}_n^{\text{GeneralLIME}}$ returned by GeneralLIME both tend to the same solution, where 
\[
\*w^{\text{LIME}} = \*w^{\text{GeneralLIME}} = \mbe_{\*z\sim \Tilde{\mbp}}[(\*z + \beta_2 \*1)f_{\*x}(\*z)], b^{\text{LIME}} = b^{\text{GeneralLIME}} = \mbe_{\*z\sim \Tilde{\mbp}}[\beta_2\|\*z\|_0 + \beta_1)f_{\*x}(\*z)], 
\]
where $\beta_1 = 1 + de^{\frac{1}{\sigma^2}},\beta_2 = -1 - e^{\frac{1}{\sigma^2}}$. 

If $\lambda = 0$, $\forall \epsilon, \delta \in (0,1)$, when $n = \Omega(d^5 e^{\frac{4}{\sigma^2}}\epsilon^{-2}\log(8d/\delta))$, we have $\mbp(\|\*w_n^{\text{LIME}} -\*w^{\text{LIME}} \| \geq \epsilon) \geq 1- \delta $ and $\mbp(\|\*w_n^{\text{GeneralLIME}} -\*w^{\text{GeneralLIME}} \| \geq \epsilon) \geq 1- \delta $
\end{proposition}
\begin{proof}
We first show the expression of $\*w^{\text{LIME}}, b^{\text{LIME}}$ and then prove concentration.

\textbf{Expression of limit. }Suppose we have i.i.d. samples $\{\*z_i\}_{i=1}^n$ drawn from distribution $\Tilde{\mbp}$. The official implementation of LIME first fit the intercept and then solve a Ridge regression problem to obtain feature attribution. Therefore, in order to match the implementation, we will add one dimension which is always equals to 1 before the first dimension of each sample $\*z_i$, i.e., $\*z_{i,0} = 1, \forall i=1,\cdots, n$. We also add one dimension representing intercept before the first dimension of $ \hat{\*w}_n^{\text{GeneralLIME}}$.

 Then 
\begin{equation}
   {\*w}_n^{\text{GeneralLIME}} = \mathop{\arg \min}_{\*v} \sum_{i=1}^n(f_{\*x}(\*z_i) - \*v^\top \*z_i)^2 + \lambda \|\*v\|_2^2 = \mathop{\arg \min}_{\*v} \frac{1}{n}\sum_{i=1}^n(f_{\*x}(\*z_i) - \*v^\top \*z_i)^2 + \frac{1}{n}\lambda \|\*v\|_2^2 
\end{equation}
Let $L_{\*x}(\*v | \*z_1,\cdots, \*z_n) = \frac{1}{n}\sum_{i=1}^n(f_{\*x}(\*z_i) - \*v^\top \*z_i)^2 + \frac{1}{n}\lambda \|\*v\|_2^2 $, then by taking the derivative of $L_{\*x}$ w.r.t. $\*v$ and equating it to zero, we have 
\[
\*v = \bigg(\frac{1}{n}\sum_{i=1}^n \*z_i\*z_i^\top + \frac{\lambda}{n}\*I \bigg)^{-1}\bigg(\frac{1}{n}\sum_{i=1}^n \*z_i f_{\*x}(\*z_i)\bigg)
\]
Denote $\*Z = (\*z_1, \cdots, \*z_n), \*F = [f_{\*x}(\*z_1), \cdots, f_{\*x}(\*z_n)]^\top$ and $\*\Sigma_n = \frac{1}{n}\*Z\*Z^\top + \frac{\lambda}{n}\*I, \*\Gamma_n = \frac{1}{n}\*Z \*F$, we have 
\[
{\*w}_n^{\text{GeneralLIME}} = \bigg(\frac{1}{n}\*Z\*Z^\top + \frac{\lambda}{n}\*I\bigg)^{-1} \frac{1}{n}\*Z \*F = \*\Sigma_n^{-1} \*\Gamma_n
\]
\[
\*\Sigma_n = \begin{bmatrix}
\frac{1}{n} \sum_i 1 + \frac{\lambda}{n} & \frac{1}{n}\sum_i \*z_{i1} & \frac{1}{n}\sum_i \*z_{i2}& \cdots & \frac{1}{n}\sum_i \*z_{id} \\ 
\frac{1}{n}\sum_i \*z_{i1} & \frac{1}{n}\sum_i \*z_{i1}^2  + \frac{\lambda}{n}& \frac{1}{n}\sum_i \*z_{i1}\*z_{i2} & \cdots & \frac{1}{n}\sum_i \*z_{i,1}\*z_{id} \\ 
\frac{1}{n}\sum_i \*z_{i2} & \frac{1}{n}\sum_i \*z_{i1}\*z_{i2} & \frac{1}{n}\sum_i \*z_{i2}^2  + \frac{\lambda}{n}&\cdots & \frac{1}{n}\sum_i \*z_{i2}\*z_{id} \\ 
\vdots & \vdots & \vdots & \ddots & \vdots \\ 
\frac{1}{n}\sum_i \*z_{id} & \frac{1}{n}\sum_i \*z_{i1}\*z_{id} & \frac{1}{n}\sum_i \*z_{i2}\*z_{id} &\cdots & \frac{1}{n}\sum_i \*z_{id}^2  + \frac{\lambda}{n}\\ 
\end{bmatrix}
\]
By taking $n\to\infty$, we have 
\[
\*\Sigma_n \to \*\Sigma = \begin{bmatrix}
    1 & \alpha_1 & \alpha_1 & \cdots & \alpha_1 \\ 
    \alpha_1 & \alpha_1 & \alpha_2 & \cdots & \alpha_2 \\ 
    \alpha_1 & \alpha_2 & \alpha_1 & \cdots & \alpha_2 \\ 
    \vdots & \vdots & \vdots & \ddots & \vdots \\ 
   \alpha_1 & \alpha_2 & \alpha_2 & \cdots & \alpha_1 \\  
\end{bmatrix}, \*\Gamma_n \to \*\Gamma = \begin{bmatrix}
    \mbe_{\*z\sim \Tilde{\mbp}}[f_{\*x}(\*z)] \\ 
    \mbe_{\*z\sim \Tilde{\mbp}}[z_{1}f_{\*x}(\*z)] \\
    \cdots \\ 
    \mbe_{\*z\sim \Tilde{\mbp}}[z_{d}f_{\*x}(\*z)] \\
\end{bmatrix}
\]
where
\[
\begin{split}
    \alpha_1 & = \mbe_{\*z_i \sim \Tilde{\mbp}}[z_{i1}], \forall i \\ 
    & = \sum_{k=0}^d \mbe(z_{i1} | \|\*z_i\|_0 = k) \mbp(\|\*z_{i}\|_0 = k) \\ 
    & = \sum_{k=0}^d \mbp(z_{i1} = 1 | \|\*z_i\|_0 = k) \mbp(\|\*z_{i}\|_0 = k) \\ 
    &  = \sum_{k=0}^d \frac{k}{d} \cdot \frac{\binom{d}{k}e^{\frac{k}{\sigma^2}}}{(1 + e^\frac{1}{\sigma^2})^d}\\
    & = \sum_{k=1}^d \frac{\binom{d-1}{k-1}e^{\frac{k}{\sigma^2}}}{(1 + e^\frac{1}{\sigma^2})^d}\\ 
    & = \sum_{k=1}^d \frac{\binom{d-1}{k-1}e^{\frac{k-1}{\sigma^2}}}{(1 + e^\frac{1}{\sigma^2})^d} e^{\frac{1}{\sigma^2}}\\ 
    & = \frac{(1 + e^\frac{1}{\sigma^2})^{d-1}}{(1 + e^\frac{1}{\sigma^2})^d} e^{\frac{1}{\sigma^2}}\\ 
    & = \frac{e^{\frac{1}{\sigma^2}}}{1 + e^\frac{1}{\sigma^2}} 
\end{split}
\]
Similarly, 
\[
\begin{split}
    \alpha_2 & = \mbe_{\*z_i \sim \Tilde{\mbp}}[z_{i1}z_{i2}], \forall i \\ 
    & = \sum_{k=0}^d \mbe[z_{i1}z_{i2} | \|\*z_i\|_0 = k] \mbp(\|\*z_{i}\|_0 = k) \\ 
    & = \sum_{k=0}^d \mbp(z_{i1} = 1, z_{i2}=1 | \|\*z_i\|_0 = k) \mbp(\|\*z_{i}\|_0 = k) \\ 
    &  = \sum_{k=2}^d \frac{k(k-1)}{d(d-1)} \cdot \frac{\binom{d}{k}e^{\frac{k}{\sigma^2}}}{(1 + e^\frac{1}{\sigma^2})^d}\\
    & = \sum_{k=2}^d \frac{\binom{d-2}{k-2}e^{\frac{k}{\sigma^2}}}{(1 + e^\frac{1}{\sigma^2})^d}\\ 
    & = \sum_{k=2}^d \frac{\binom{d-2}{k-2}e^{\frac{k-2}{\sigma^2}}}{(1 + e^\frac{1}{\sigma^2})^d} e^{\frac{2}{\sigma^2}}\\ 
    & = \frac{(1 + e^\frac{1}{\sigma^2})^{d-2}}{(1 + e^\frac{1}{\sigma^2})^d} e^{\frac{2}{\sigma^2}}\\ 
    & = \frac{e^{\frac{2}{\sigma^2}}}{(1 + e^\frac{1}{\sigma^2})^2} = \alpha_1^2 
\end{split}
\]
Let $A = [1], B = \alpha_1 \*1^\top, C = \alpha_1 \*1, D = \alpha_2 \*1\*1^\top + (\alpha_1 - \alpha_2) \*I,$ we have 
\[
\*\Sigma = \begin{bmatrix}
    A & B \\ 
    C & D \\ 
\end{bmatrix}
\]
Applying Theorem 2.2 in \cite{lu2002inverses}, we can get 
\[
\*\Sigma^{-1} = \begin{bmatrix}
    \beta_1 & \beta_2 & \cdots & \beta_2 \\ 
    \beta_2 & \beta_3 & \cdots & 0 \\ 
    \vdots & \vdots & \ddots & 0\\ 
    \beta_2 & 0 & \cdots & \beta_3 \\ 
    \end{bmatrix}
\]
where 
\[
\beta_3 = \frac{\alpha_1 + (d-1) \alpha_2}{\alpha_1 - \alpha_2} = \frac{1+(d-1)\alpha_1}{1-\alpha_1}, \beta_1 = - \frac{\alpha_1}{\alpha_1 - \alpha_2} = -\frac{1}{1 - \alpha_1} = -(1 + e^{\frac{1}{\sigma^2}})
\]
\[
\beta_2 = \frac{1}{\alpha_1 - \alpha_2}
\]
Multiplying $\*\Sigma^{-1}$ and $\*\Gamma$, we have 
\[
\*\Sigma^{-1}\*\Gamma = \begin{bmatrix}
    \beta_3 \mbe_{\*z\sim \Tilde{\mbp}}[f_{\*x}(\*z)] + \beta_1 \sum_{k=1}^d \mbe_{\*z\sim \Tilde{\mbp}}[z_{k}f_{\*x}(\*z)] \\
    \beta_1\mbe_{\*z\sim \Tilde{\mbp}}[f_{\*x}(\*z)] + \beta_2\mbe_{\*z\sim \Tilde{\mbp}}[z_{1}f_{\*x}(\*z)] \\
\vdots \\ 
\beta_1\mbe_{\*z\sim \Tilde{\mbp}}[f_{\*x}(\*z)] + \beta_2\mbe_{\*z\sim \Tilde{\mbp}}[z_{d}f_{\*x}(\*z)] \\
\end{bmatrix}
\]
Hence, 
\[
\*w^*_j =  \beta_1\mbe_{\*z\sim \Tilde{\mbp}}[f_{\*x}(\*z)] +  \beta_2\mbe_{\*z\sim \Tilde{\mbp}}[z_{j}f_{\*x}(\*z)], \forall j=1,\cdots, d
\]

Since \autoref{eq:eqivalence} has already show the equivalence of LIME and GeneralLIME in the limit, ${\*w}_n^{\text{LIME}}$ also converges to $\*w^*$.

\textbf{Concentration of LIME and GeneralLIME.} Since we have already obtained the limit of ${\*w}_n^{\text{LIME}}$ and $\lambda=0$, instead of computing LIME explanation by solving a Ridge regression problem, we can use finite sample approximation to integrals in ${\*w}^{\text{LIME}}$. 
Then 
\[
{\*w}_n^{\text{GeneralLIME}} = {\*w}_n^{\text{LIME}} = \frac{1}{n}\sum_{i=1}^n (\beta_2 \*z_i + \beta_1 \*1) f_{\*x}(\*z_i)
\]
Let $\*g_i = (\beta_2 \*z_i + \beta_1 \*1) f_{\*x}(\*z_i)$, then we have 
\[
\|\*g_i\| \leq \|\beta_2 \*z_i + \beta_1 \*1\| \leq (\beta_2+\beta_1)\sqrt{d + 1} = (1 + e^{-\frac{1}{\sigma^2}})\sqrt{d+1}
\]
By matrix form of Hoeffding's inequality \cite{tropp2015introduction, garreau2021does}, we have $\forall t > 0$
\[
\mbp(\|\frac{1}{n}\sum_{i=1}^n \*g_i - \*w\| \geq t) \leq 2 (d+1) \exp(-\frac{nt^2}{4((1 + e^{-\frac{1}{\sigma^2}})\sqrt{d+1})^2})
\]
Therefore, $\forall \epsilon >0, \delta \in (0,1)$, if $n \geq \Omega(\epsilon^{-2}d^2(1+e^{-\frac{1}{\sigma^2}})^2 \log(8d/\delta))$, we have 
\[
\mbp(\|\frac{1}{n}\sum_{i=1}^n \*g_i - \*w\| \geq \epsilon) \leq \delta 
\]
\end{proof}

\subsection{Proof of \cref{thm:over_regularization}}

\begin{theorem}
    Suppose in LIME we have samples $\{\*z_i\}_{i=1}^n \sim \text{Uni}(\{0,1\}^d)$. For any $t >0, \delta \in (0,1)$, if the sample size in LIME satisfies 
    \[
    n = O\bigg(\lambda t \bigg(\frac{2e^{\frac{1}{\sigma^2}}}{1+e^{\frac{1}{\sigma^2}}}\bigg)^{d-1}\sqrt{\log\frac{1}{\delta}}\bigg),
    \]
    we have $\mbp(\frac{1}{n}\sum_{i=1}^n \pi(\*z_i)\sum_j z_{ij}/d < \frac{\lambda }{n}t) \geq 1 - \delta $.
    
    Suppose in GeneralLIME we have samples $\{\*z_i\}_{i=1}^n \sim \Tilde{\mbp}$. For any $t >0, \delta \in (0,1)$, if  the sample size in GeneralLIME satisfies 
    \[
    n = O\bigg(\lambda t \sqrt{\log\frac{1}{\delta}}\bigg),
    \]
    we have $\mbp(\frac{1}{n}\sum_i\|\bz_i\|_0/d  < \frac{\lambda }{n}t) \geq  1-\delta.$
\end{theorem}

\begin{lemma}\label[lemma]{lemma:concentrate_orig}
Suppose we have samples $\{\*z_i\}_{i=1}^n \sim \text{Uni}(\{0,1\}^d)$.Let $\alpha_0 = \mbe_{\*z \sim \text{Uni}(\{0,1\}^d)}[\pi(\*z) \|\*z\|_0/d]$.    For any $t >0, \delta \in (0,1)$, if $n \leq \frac{2\lambda t \alpha_0 - \sqrt{2\lambda t\alpha_0 \log \frac{1}{\delta}}}{2\alpha_0^2}$, for LIME explanation, we have 
    \[
    \mbp(\frac{1}{n}\sum_{i=1}^n \pi(\*z_i)\sum_j z_{ij}/d < \frac{\lambda }{n}t) \geq 1 - \delta 
    \]
\end{lemma}

\begin{proof}
    Let $y_i = \pi(\*z_i)\sum_j z_{ij}/d, \hat{y} = \frac{1}{n}\sum_i y_i$, then 

    \[
        \alpha_0 = \mbe[y_i] = \sum_{k=0}^{d}\frac{k}{d} \frac{\binom{d}{k}}{2^d} e^{\frac{k-d}{\sigma^2}   }  =\sum_{k=0}^{d}\frac{\binom{d-1}{k-1}}{2^d} e^{\frac{k-d}{\sigma^2}   } = \frac{1}{2}\bigg(\frac{1 + e^{-\frac{1}{\sigma^2}}}{2}\bigg)^{d-1}
    \]

    For $n \geq \frac{\lambda  t}{\alpha_0}$
    \[
        \hat{y} < \frac{\lambda }{n}t \Longleftrightarrow \hat{y} - \alpha_0 < \frac{\lambda t}{n} - \alpha_0 < 0
    \]
Since $0\leq y_i \leq 1$, thus by Hoeffding inequality, we have 
    \[
    \begin{split}
        \mbp( \hat{y} - \alpha_0 < \frac{\lambda t}{n} - \alpha_0)   & \leq \exp\big(-2n(\frac{\lambda t}{n} - \alpha_0)^2\big)\\ 
    \end{split}
    \]
    Because
    \[
        \begin{split}
             & n \geq \frac{4\lambda t \alpha_0 + \log\frac{1}{\delta} + \sqrt{8\lambda t\alpha_0 \log \frac{1}{\delta} + 16 \lambda^2 t^2 \alpha_0^2 + \log^2\frac{1}{\delta} - 16\lambda^2 t^2\alpha_0^2}}{4\alpha_0^2}\\ 
            \Longleftrightarrow& 2\alpha_0^2 n^2 - (4\lambda t\alpha_0 +\log\frac{1}{\delta})n + 2\lambda^2 t^2 \geq 0 \\ 
            \Longleftrightarrow& \frac{2\alpha_0^2(n - \frac{\lambda t}{\alpha_0})^2}{n} \geq \log\frac{1}{\delta}\\ 
            \Longleftrightarrow &  \exp\big(-2n(\frac{\lambda t}{n} - \alpha_0)^2\big) \leq \delta \\ 
        \end{split}
    \]
    That is 
    \[
    \mbp(\frac{1}{n}\sum_{i=1}^n \pi(\*z_i)\sum_j z_{ij}/d < \frac{\lambda }{n}t) \geq 1 - \delta 
    \]

\end{proof}

\begin{lemma}\label[lemma]{lemma:concentrate_GeneralLIME}
    Suppose we have samples $\{\*z_i\}_{i=1}^n \sim \Tilde{\mbp}$. Let $\gamma = \mbe_{\*z\sim \Tilde{\mbp}}[\|\bz\|_0/d]$. For any $t >0, \delta \in (0,1)$, if $n \leq \frac{2\lambda t \gamma - \sqrt{2\lambda t\gamma \log \frac{1}{\delta}}}{2\gamma^2}$, we have 
    \[
    \mbp(\frac{1}{n}\sum_i\|\bz_i\|_0/d  < \frac{\lambda }{n}t) \geq  1-    \delta 
    \]
\end{lemma}

\begin{proof}
Let $w_i = |\bz_i|/d, \hat{w} = \frac{1}{n}\sum_i w_i $. The distribution of $w_i$ is as follows:
    \[
    \mbp(w_i = k/d) = \frac{\binom{d}{k}e^{\frac{k}{\sigma^2}}}{(1+e^{\frac{1}{\sigma^2}})^d}, 
    \]

    \[
        \mbe[w_i] = \sum_{k=0}^{d}\frac{k}{d}\frac{\binom{d}{k}e^{\frac{k}{\sigma^2}}}{(1+e^{\frac{1}{\sigma^2}})^d} =\sum_{k=0}^{d}\frac{\binom{d-1}{k-1}e^{\frac{k}{\sigma^2}}}{(1+e^{\frac{1}{\sigma^2}})^d} = \frac{1}{1 + e^{-\frac{1}{\sigma^2}}} = \gamma, \mbe[\hat{w}] = \gamma
    \]

    For $n \leq \frac{2\lambda t \gamma - \sqrt{2\lambda t\gamma \log \frac{1}{\delta}}}{2\bGamma^2}\leq \frac{\lambda  t}{\gamma}$
    \[
        \hat{w} > \frac{\lambda }{n}t \Longleftrightarrow \hat{w} - \gamma > \frac{\lambda t}{n} - \gamma > 0
    \]
Since $0\leq y_i \leq 1$, thus by Hoeffding inequality, we have 
    \[
    \begin{split}
        \mbp( \hat{w} - \gamma > \frac{\lambda t}{n} - \gamma)   & \leq \exp\big(-2n(\frac{\lambda t}{n} - \gamma)^2\big)\\ 
    \end{split}
    \]
    Because
    \[
        \begin{split}
             & n < \frac{2\lambda t \gamma - \sqrt{2\lambda t\gamma \log \frac{1}{\delta}}}{2\gamma^2} \leq \frac{4\lambda t \gamma + \log\frac{1}{\delta} - \sqrt{8\lambda t\gamma \log \frac{1}{\delta} + 16 \lambda^2 t^2 \gamma^2 + \log^2\frac{1}{\delta} - 16\lambda^2 t^2\gamma^2}}{4\gamma^2}\\ 
            \Longleftrightarrow& 2\gamma^2 n^2 - (4\lambda t\gamma +\log\frac{1}{\delta})n + 2\lambda^2 t^2 \geq 0 \\ 
            \Longleftrightarrow& \frac{2\gamma^2(n - \frac{\lambda t}{\gamma})^2}{n} \geq \log\frac{1}{\delta}\\ 
            \Longleftrightarrow &  \exp\big(-2n(\frac{\lambda t}{n} - \gamma)^2\big) \leq \delta \\ 
        \end{split}
    \]
That is 
    \[
     \mbp(\frac{1}{n}\sum_i\|\bz_i\|_0/d  < \frac{\lambda }{n}t) \geq  1-    \delta 
    \]
\end{proof}

Note that the sample complexity bound has the same form as that in \cref{lemma:concentrate_orig} but with $\gamma$ in stead of $\alpha_0$. This small change actually makes huge difference on the sample complexity bounds. This is due to the fact that $\gamma$ is lower bounded by a positive number that is independent of $e^{-\frac{1}{\sigma^2}}$.
\[
\frac{1}{2} \leq \gamma = \frac{1}{1 + e^{-\frac{1}{\sigma^2}}} \leq 1
\]

When $\sigma$ is small, the sample complexity bound does not grow exponentially as it is in the original LIME. 

\subsection{Proof of \cref{thm:close_to_zero}}

\begin{theorem}
For any $\epsilon , \delta \in (0,1)$, when sample size used in LIME satisfies
\[
n = O\bigg(\lambda \epsilon d^{-0.5}\bigg(\frac{2e^{\frac{1}{\sigma^2}}}{1+e^{\frac{1}{\sigma^2}}}\bigg)^d\sqrt{\log\frac{1}{\delta}}\bigg),
\]
we have LIME explanation is close to zero with high probability, i.e., $\mathbb{P}(\|\bw^{\text{LIME}}_n\| < \epsilon) \geq 1- \delta$.

When sample size used in GeneralLIME satisfies
\[
n = O\bigg(\lambda \epsilon d^{-1}\sqrt{\log\frac{1}{\delta}}\bigg),
\]
we have GeneralLIME explanation is close to zero with high probability, i.e., $\mathbb{P}(\|\bw^{\text{GeneralLIME}}_n\| < \epsilon) \geq 1- \delta$.
\end{theorem}
In order to prove this theorem, we first show two lemmas which will be proved at the end of this section. And the result of \cref{thm:close_to_zero} is just the combination of them. 

\begin{lemma}\label[lemma]{lemma:lime_weight_close_to_zero}
    Suppose we have $n$ samples $\{\bz_1, \cdots, \bz_n\}, \bz_i \sim \text{Uni}(\{0,1\}^d)$ and $\bw^{\text{LIME}}_n$ is the minimizer of LIME given these samples computed from \autoref{eq:ori_lime}. 
    Then $\forall \epsilon, \delta \in (0,1)$, if $n \leq \frac{2\lambda \epsilon \mbe[\pi(\*z_i)] - \sqrt{2\lambda \epsilon\mbe[\pi(\*z_i)]\sqrt{d} \log \frac{1}{\delta}}}{2\sqrt{d}\mbe[\pi(\*z_i)]^2}$, we have  
    $\mathbb{P}(\|\bw^{\text{LIME}}_n\| < \epsilon) \geq 1- \delta$.
\end{lemma}
\begin{lemma}\label[lemma]{lemma:GeneralLIME_weight_close_to_zero}
    Suppose we have $n$ samples $\{\bz_1, \cdots, \bz_n\}, \bz_i \sim \Tilde{\mbp}$ and $\bw^{\text{GeneralLIME}}_n$ is the minimizer of GeneralLIME given these samples computed from \autoref{eq:eqivalence}. 
    Then $\forall \epsilon, \delta \in (0,1)$, if $n < \frac{2\lambda \epsilon \mbe[\sqrt{\|\*z_i\|_0}] - \sqrt{2\lambda \epsilon\mbe[\sqrt{\|\*z_i\|_0}]\sqrt{d} \log \frac{1}{\delta}}}{2\mbe[\sqrt{\|\*z_i\|_0}]^2}$, we have  
    $\mbp(\|\bw^{\text{GeneralLIME}}_n\| \leq \epsilon)\geq 1 - \delta$.
\end{lemma}

\cref{lemma:lime_weight_close_to_zero} shows that LIME explanation is close to zero when the sample size $n \leq \frac{2\lambda \epsilon \mbe[\pi(\*z_i)] - \sqrt{2\lambda \epsilon\mbe[\pi(\*z_i)]\sqrt{d} \log \frac{1}{\delta}}}{2\sqrt{d}\mbe[\pi(\*z_i)]^2}$ which is of order $O(\lambda \epsilon d^{-0.5}\mbe^{-1}[\pi(\*z_i)]\log^{0.5}\frac{1}{\delta})$. However, $\mbe^{-1}[\pi(\*z_i)] = (\frac{2e^{\frac{1}{\sigma^2}}}{1+e^{\frac{1}{\sigma^2}}})^d$ which grows exponentially and when $\sigma$ is small, it is close to $2^d$. When $\sigma$ is small, we need more samples to found solution that are separated from zero. 

On the other hand,\cref{lemma:GeneralLIME_weight_close_to_zero} shows that GeneralLIME explanation is close to zero with high probability when $n < \frac{2\lambda \epsilon \mbe[\sqrt{\|\*z_i\|_0}] - \sqrt{2\lambda \epsilon\mbe[\sqrt{\|\*z_i\|_0}]\sqrt{d} \log \frac{1}{\delta}}}{2\mbe[\sqrt{\|\*z_i\|_0}]^2}$. However, 
\[
\sqrt{\sum_{k=0}^d {k}\frac{\binom{d}{k}e^{\frac{k}{\sigma}}}{(1 + e^{\frac{1}{\sigma^2}})^2}} = \sqrt{\frac{d}{1 + e^{-\frac{1}{\sigma^2}}}} \leq \mbe[\sqrt{\|\*z_i\|_0}] = \sum_{k=0}^d \sqrt{k}\frac{\binom{d}{k}e^{\frac{k}{\sigma}}}{(1 + e^{\frac{1}{\sigma^2}})^2} \leq \sum_{k=0}^d \frac{k\binom{d}{k}e^{\frac{k}{\sigma}}}{(1 + e^{\frac{1}{\sigma^2}})^2} = \frac{d}{1 + e^{-\frac{1}{\sigma^2}}}
\]
then
\[
\frac{1}{d} \leq \frac{1+e^{-\frac{1}{\sigma^2}}}{d}\leq \mbe^{-1}[\sqrt{\|\*z_i\|_0}] \leq \sqrt{\frac{1 + e^{-\frac{1}{\sigma^2}}}{d}} \leq \sqrt{\frac{2}{d}}
\]
which grows much slower than $\mbe^{-1}[\pi(\*z_i)]$ and $\sigma$ has little effect on the bound. 

Comparing these two lemmas, we can conclude that if we only have limited samples, the solution found by LIME is close to zero while that found by GeneralLIME is much more meaningful. 

\begin{proof}[Proof of \cref{lemma:lime_weight_close_to_zero}]
Since 
\[
    \bw^{\text{LIME}}_n = {\bSigma}_n^{-1} {\bGamma}_n     
\]
we have 
\[
\| \bw^{\text{LIME}}_n\| \leq \epsilon \Longleftrightarrow \|\bSigma_n^{-1}\bGamma_n\| \leq \epsilon     
\]

Since $\bz_i \in \{0,1\}^d$ and $\pi(\bz_i)> 0, \forall i$, the norm of $\bGamma_n$ can be easily bounded 
\[
\|\bGamma_n\| \leq \|[\frac{1}{n}\sum_i \pi(\*z_i) z_{i,1}, \cdots, \frac{1}{n}\sum_i \pi(\*z_i) z_{i,d}]^\top \| \leq \frac{1}{n}\sum_i \pi(\*z_i) \sqrt{d}    
\]
Then 
\[
\begin{split}
   & \|\bSigma_n^{-1}\bGamma_n\| \leq \|\bSigma_n^{-1}\|_2\|\bGamma_n\|_2 \leq \|\bSigma_n^{-1}\|_2 \cdot \frac{1}{n}\sum_i \pi(\*z_i) \sqrt{d} \leq \epsilon \\ 
   & \Rightarrow \|\bSigma_n^{-1}\| \leq \frac{n\epsilon }{\sum_i \pi(\*z_i) \sqrt{d}}
\end{split}
\]

It is easy to see that $\bSigma_n$ is symmetric and positive definite so that its eigenvalues are all positive. We have $\lambda_{\min}(\bSigma_n) = \lambda_{\min}(\frac{1}{n}\sum_i \pi(\*z_i)\*z_i\*z_i^\top) + \frac{\lambda}{n} $. Therefore, 
\[
   \begin{split}
    &\|\bSigma_n^{-1}\|_2 = \frac{1}{\lambda_{\min}(\frac{1}{n}\sum_i \pi(\*z_i)\*z_i\*z_i^\top) + \frac{\lambda}{n} }\leq \frac{n\epsilon }{\sum_i \pi(\*z_i) \sqrt{d}} \\ 
    & \Rightarrow\lambda_{\min}(\frac{1}{n}\sum_i \pi(\*z_i)\*z_i\*z_i^\top) + \frac{\lambda}{n} = \frac{\lambda}{n}\geq \frac{ \sum_i \pi(\*z_i) \sqrt{d}}{ n\epsilon} 
   \end{split}
\]

Then we can bound $\mathbb{P}(\frac{ \sum_i \pi(\*z_i) \sqrt{d}}{\epsilon}  \leq \lambda ) = \mathbb{P}(\sum_i \pi(\*z_i) \leq \frac{\lambda \epsilon}{\sqrt{d}}) $ by Hoeffding inequality,
\[
        \begin{split}
             & n < \frac{2\lambda \epsilon \mbe[\pi(\*z_i)] - \sqrt{2\lambda \epsilon\mbe[\pi(\*z_i)]\sqrt{d} \log \frac{1}{\delta}}}{2\sqrt{d}\mbe[\pi(\*z_i)]^2} \\
             & \leq \frac{4\lambda \epsilon\mbe[\pi(\*z_i)] /\sqrt{d}+ \log\frac{1}{\delta} - \sqrt{8\frac{\lambda \epsilon\mbe[\pi(\*z_i)]}{\sqrt{d}}\log \frac{1}{\delta} + 16 \lambda^2 \epsilon^2 \mbe[\pi(\*z_i)]^2/d + \log^2\frac{1}{\delta} - 16\lambda^2 \epsilon^2\mbe[\pi(\*z_i)]^2/d}}{4\mbe[\pi(\*z_i)]^2}\\ 
            \Longleftrightarrow& 2\mbe[\pi(\*z_i)]^2 n^2 - (4\lambda \epsilon\mbe[\pi(\*z_i)]/\sqrt{d} +\log\frac{1}{\delta})n + 2\lambda^2 \epsilon^2/d \geq 0 \\ 
            \Longleftrightarrow& \frac{2\mbe[\pi(\*z_i)]^2(n - \frac{\lambda \epsilon}{\mbe[\pi(\*z_i)]\sqrt{d}})^2}{n} \geq \log\frac{1}{\delta}\\ 
            \Longleftrightarrow &  \exp\big(-2n(\frac{\lambda \epsilon}{n\sqrt{d}} - \mbe[\pi(\*z_i)])^2\big) \leq \delta \\ 
        \end{split}
    \]
\[
 \begin{split}
    \mathbb{P}(\sum_i \pi(\*z_i) \geq \frac{\lambda \epsilon}{\sqrt{d}})  & =  \mathbb{P}(\frac{1}{n}\sum_i \pi(\*z_i) - \mbe[{\pi(\*z_i)}]\geq \frac{\lambda \epsilon}{n\sqrt{d}} - \mbe[{\pi(\*z_i)}]) \\ 
    & \leq \exp(-2n( \frac{\lambda \epsilon}{n\sqrt{d}} - \mbe[{\pi(\*z_i)}])^2)
 \end{split}
\]
If $n \leq \frac{2\lambda \epsilon \mbe[\pi(\*z_i)] - \sqrt{2\lambda \epsilon\mbe[\pi(\*z_i)]\sqrt{d} \log \frac{1}{\delta}}}{2\sqrt{d}\mbe[\pi(\*z_i)]^2} $, we have 
\[
    \mathbb{P}(\sum_i \pi(\*z_i) \geq \frac{\lambda \epsilon}{\sqrt{d}})  \leq \delta 
\]
that is 
\[
    \mathbb{P}(\sum_i \pi(\*z_i) \leq \frac{\lambda \epsilon}{\sqrt{d}})  \geq 1- \delta 
\]
and as a consequence, 
\[
\mathbb{P}(\|\bw^{\text{LIME}}_n\| \leq \epsilon) \geq 1 - \delta     
\]
However, is the sample complexity bound meaningful? To see why is it meaningful, we need to bound $\mathbb{E}_{\bz}[\pi(\bz)]$ 

\[
C = \mathbb{E}_{\bz}[\pi(\bz)] = \sum_{k=0}^d \frac{\tbinom{d}{k}}{2^d} e^{\frac{k-d}{{\sigma}^2}} \leq \frac{2^d - 1}{2^d} e^{-\frac{1}{{\sigma}^2}} + \frac{1}{2^d}
\]

\[
\mathbb{E}_{\bz}[\pi(\bz)] = \sum_{k=0}^d \frac{\tbinom{d}{k}}{2^d} e^{\frac{k-d}{{\sigma}^2}} \geq \frac{2^d - 1}{2^d} e^{-\frac{d}{{\sigma}^2}} + \frac{1}{2^d}
\]

And it is easy to prove that $C$ is increasing w.r.t ${\sigma}$ when ${\sigma} > 0$ is close to 0. Hence, when ${\sigma}$ becomes small, $C$ becomes small and the sample complexity bound becomes large. One implication from this is that when ${\sigma}$ is small, we need more samples to have $\|\bw^*\|\geq \epsilon$ w.p. $1-\delta$.
\end{proof}

A direct corollary from this result is that 
\[
\mathbb{P}(|(\bw^{\text{LIME}}_n)_i - (\bw^{\text{LIME}}_n)_j| > 2\epsilon ) \leq \delta     
\]
\begin{proof}
    If $|(\bw^{\text{LIME}}_n)_i - (\bw^{\text{LIME}}_n)_j| > 2\epsilon$, then we must have that at least one of $|(\bw^{\text{LIME}}_n)_i| > \epsilon$ and $|  (\bw^{\text{LIME}}_n)_j| > \epsilon$ holds. This leads to $\|\bw^{\text{LIME}}_n\|\geq \epsilon$ which is a contradiction.
    
\end{proof}

\begin{proof}[Proof of \cref{lemma:GeneralLIME_weight_close_to_zero}]
Since 
\[
    \bw^{\text{GeneralLIME}}_n = {\bSigma}_n^{-1} {\bGamma}_n     
\]
we have 
\[
\| \bw^{\text{GeneralLIME}}_n\| \leq \epsilon \Longleftrightarrow \|\bSigma_n^{-1}\bGamma_n\| \leq \epsilon     
\]

Since $\bz_i \in \{0,1\}^d$ , the norm of $\bGamma_n$ can be easily bounded 
\[
\begin{split}
    \|\bGamma_n\| \leq \|[\frac{1}{n}\sum_i z_{i,1}, \cdots, \frac{1}{n}\sum_i z_{i,d}]^\top \| & = \bigg[\sum_j \big(\frac{1}{n}\sum_i z_{ij})^2\bigg]^{-\frac{1}{2}}\\ 
    &\leq \bigg[\sum_j \frac{1}{n}\sum_iz_{ij}^2\bigg]^{-\frac{1}{2}} \\
    & = \bigg[\sum_j \frac{1}{n}\sum_iz_{ij}\bigg]^{-\frac{1}{2}} \\ 
    & = \bigg[\frac{1}{n}\sum_i \|\*z_i\|_0\bigg]^{-\frac{1}{2}} \\ 
    & \leq \frac{1}{n}\sum_i \|\*z_i\|_0^{-\frac{1}{2}}
\end{split}  
\]
Then 
\[
\begin{split}
   &  \|\bSigma_n^{-1}\bGamma_n\| \leq \|\bSigma_n^{-1}\|_2\|\bGamma_n\|_2 \leq \|\bSigma_n^{-1}\|_2 \cdot  \frac{1}{n}\sum_i \|\*z_i\|_0^{-\frac{1}{2}} \leq \epsilon\\ 
   & \Rightarrow \|\bSigma_n^{-1}\| \leq \frac{\epsilon}{\frac{1}{n}\sum_i \|\*z_i\|_0^{-\frac{1}{2}}}
\end{split}
\]

It is easy to see that $\bSigma_n$ is symmetric and positive definite so that its eigenvalues are all positive. We have $\lambda_{\min}(\bSigma_n) = \lambda_{\min}(\frac{1}{n}\sum_i \*z_i\*z_i^\top) + \frac{\lambda}{n} $. Therefore, 
\[
   \begin{split}
    &\|\bSigma_n^{-1}\|_2 = \frac{1}{\lambda_{\min}(\frac{1}{n}\sum_i \*z_i\*z_i^\top) + \frac{\lambda}{n} }\leq \frac{\epsilon}{\frac{1}{n}\sum_i \|\*z_i\|_0^{-\frac{1}{2}}} \\ 
    & \Rightarrow  \lambda_{\min}(\frac{1}{n}\sum_i \*z_i\*z_i^\top) + \frac{\lambda}{n} = \frac{\lambda}{n}\geq \frac{\frac{1}{n}\sum_i \|\*z_i\|_0^{-\frac{1}{2}}}{\epsilon} 
   \end{split}
\]
 Then we can bound $\mathbb{P}(\frac{ \sum_i\|\*z_i\|_0^{-\frac{1}{2}}}{\epsilon}  \leq \lambda ) = \mathbb{P}(\sum_i\|\*z_i\|_0^{-\frac{1}{2}} \leq {\lambda \epsilon}) $ by Hoeffding inequality,
\[
        \begin{split}
             & n < \frac{2\lambda \epsilon \mbe[\sqrt{\|\*z_i\|_0}] - \sqrt{2\lambda \epsilon\mbe[\sqrt{\|\*z_i\|_0}]\sqrt{d} \log \frac{1}{\delta}}}{2\mbe[\sqrt{\|\*z_i\|_0}]^2} \\
             & \leq \frac{4\lambda \epsilon\mbe[\sqrt{\|\*z_i\|_0}]+ \log\frac{1}{\delta} - \sqrt{8{\lambda \epsilon\mbe[\sqrt{\|\*z_i\|_0}]}\log \frac{1}{\delta} + 16 \lambda^2 \epsilon^2 \mbe[\sqrt{\|\*z_i\|_0}]^2 + \log^2\frac{1}{\delta} - 16\lambda^2 \epsilon^2\mbe[\sqrt{\|\*z_i\|_0}]^2}}{4\mbe[\sqrt{\|\*z_i\|_0}]^2}\\ 
            \Longleftrightarrow& 2\mbe[\sqrt{\|\*z_i\|_0}]^2 n^2 - (4\lambda \epsilon\mbe[\sqrt{\|\*z_i\|_0}] +\log\frac{1}{\delta})n + 2\lambda^2 \epsilon^2 \geq 0 \\ 
            \Longleftrightarrow& \frac{2\mbe[\sqrt{\|\*z_i\|_0}]^2(n - \frac{\lambda \epsilon}{\mbe[\sqrt{\|\*z_i\|_0}]})^2}{n} \geq \log\frac{1}{\delta}\\ 
            \Longleftrightarrow &  \exp\big(-2n(\frac{\lambda \epsilon}{n} - \mbe[\sqrt{\|\*z_i\|_0}])^2\big) \leq \delta \\ 
        \end{split}
    \]
\[
 \begin{split}
    \mathbb{P}(\sum_i \sqrt{\|\*z_i\|_0}\geq {\lambda \epsilon})  & =  \mathbb{P}(\frac{1}{n}\sum_i \sqrt{\|\*z_i\|_0}- \mbe[{\sqrt{\|\*z_i\|_0}}]\geq \frac{\lambda \epsilon}{n} - \mbe[{\sqrt{\|\*z_i\|_0}}]) \\ 
    & \leq \exp(-2n( \frac{\lambda \epsilon}{n} - \mbe[{\sqrt{\|\*z_i\|_0}}])^2)
 \end{split}
\]
If $n \leq \frac{2\lambda \epsilon \mbe[\sqrt{\|\*z_i\|_0}] - \sqrt{2\lambda \epsilon\mbe[\sqrt{\|\*z_i\|_0}] \log \frac{1}{\delta}}}{2\mbe[\sqrt{\|\*z_i\|_0}]^2} $, we have 
\[
    \mathbb{P}(\sum_i \sqrt{\|\*z_i\|_0} \geq {\lambda \epsilon})  \leq \delta 
\]
that is 
\[
    \mathbb{P}(\sum_i \sqrt{\|\*z_i\|_0}\leq {\lambda \epsilon})  \geq 1- \delta 
\]
and as a consequence, 
\[
\mathbb{P}(\|\bw^{\text{GeneralLIME}}_n\| \leq \epsilon) \geq 1 - \delta     
\]
\end{proof}

\subsection{Formulation of SmoothGrad}\label[appendix]{app:smooth-grad}

\begin{proposition}
SmoothGrad is equivalent to GeneralLIME formulation with $\mathcal{T}(\*x) = \*x$,  $\*z = \*z^\prime + \*x $ where $\*z^\prime \sim \mathcal{N}(\*0, \sigma^2 \*I)$, $\ell(f(\*z), g_{\*v}(\*z^\prime)) = (f(\*z) - g_{\*v}(\*z^\prime))^2$ and $\pi(\*z) = 1, \Omega(\*v) = 0$. 

The explanation returned by GeneralLIME for $f$ at $\*x$ with infinitely many samples under the above setting is 
\[
\*w^* = \frac{1}{\sigma^2}\mbe_{\*z^\prime\sim \mathcal{N}(\*0, \sigma^2 \*I)}[\*z^\prime f(\*z^\prime + \*x)] = \mathbb{E}_{\*z^\prime\sim \mathcal{N}(\*0, \sigma^2 \*I)}[\nabla f(\*x + \*z^\prime)]
\]
which is exactly SmoothGrad explanation. When $\sigma\to 0$, $\*w^* \to \nabla f(\*x + \*z)|_{\*z = \*0}$.
\end{proposition}

\begin{proof}

To prove this proposition, we first derive the expression of GeneralLIME explanation $\*w^*$. 

\textbf{Exact Expression of $\*\Sigma$. }$\*z_i^\prime \sim \mathcal{N}(\mathbf{0}, \sigma^2\*I), \forall i=1,\cdots, n$. In this case 
\[
\hat{\*\Sigma}_n = \begin{bmatrix}
    \frac{1}{n}\sum_k 1& \frac{1}{n}\sum_k z_{k1}^\prime & \cdots & \frac{1}{n}\sum_k z_{kd}^\prime \\ 
    \frac{1}{n}\sum_k z_{k1}^\prime & \frac{1}{n} \sum_k (z_{k1}^2)^\prime & \cdots & \frac{1}{n}\sum_k z_{l1}^\prime z_{kd}^\prime \\ 
    \vdots & \vdots & \ddots & \vdots \\ 
     \frac{1}{n}\sum_k z_{k1}^\prime &  \frac{1}{n}\sum_k z_{kd}^\prime z_{k1}^\prime & \cdots &  \frac{1}{n}\sum_k (z_{kd}^2)^\prime\\
\end{bmatrix}
\]
Then we have 
\[
\*\Sigma = \mathbb{E}_{\*z^\prime\sim \mathcal{N}(\*0, \sigma^2\*I}[\*z^\prime(\*z^\prime)^\top] = \begin{bmatrix}
    1 & 0 & \cdots & 0 \\ 
    0 & \sigma^2 & \cdots & 0 \\ 
    \vdots & \vdots & \ddots & \vdots \\ 
    0 & 0 & \cdots & \sigma^2 \\ 
\end{bmatrix}
\]
\[
\*\Sigma^{-1} = \begin{bmatrix}
    1 & 0 & \cdots & 0 \\ 
0 & \frac{1}{\sigma^2} & \cdots & 0 \\ 
    \vdots & \vdots & \ddots & \vdots \\ 
0 & 0 & \cdots & \frac{1}{\sigma^2} \\ 
\end{bmatrix}
\]
As a direct consequence, we have 
\[
\*w^* = (\*\Sigma^{-1} \*\Gamma)_{[1:d+1]} =  \frac{1}{\sigma^2}\mbe_{\*z^\prime\sim \mathcal{N}(\*0, \sigma^2 \*I)}[\*z^\prime f(\*x + \*z^\prime)]= \mathbb{E}_{\*z^\prime\sim \mathcal{N}(\*0, \sigma^2 \*I)}[\nabla f(\*x + \*z^\prime)]
\]

The last equality directly follows from Stein's lemma \cite{lin2019stein}.
\end{proof}
