# Supplementary material for: GLIME: General, Stable and Local LIME Explanation
Source: arXiv:2311.15722 source file (2023-11-27)
Supplement: Supplementary file 2 [file proofs_old.tex]

\section{Preliminary}
Consider a model $f:\mathcal{X}\to \mathcal{Y}, \mathcal{X} = [0,1]^d, \mathcal{Y} = [0,1]$ and an input to be explained $\bx\in \mathcal{X}$. The perturbed samples drawn are $\{\bz_i\}_{i=1}^n, \bz_i \in \{0,1\}^d$. We use $|\bz_i|$ to denote the number of non-zero elements in $\bz_i$. $\|\cdot\|_2$ denote the $L_2$ norm.

Original LIME: 
In the paper of LIME, the authors suggest to use L2 distance for images, so we consider the following objective function for LIME.
\begin{equation}\label{eq:lime}
    \bw^* = \mathop{\arg\min}_\bw \sum_{i=1}^n \pi(\bz_i)(f(\bz_i) - \bw^\top \bz_i)^2 + \lambda \|\bw\|^2    , \pi(\bz_i) = e^{\frac{|\bz_i| -d}{{\sigma}^2}}, \bz_i \sim \text{Uni}(\{0,1\}^d)
\end{equation}

Modified LIME: To get a perturbed sample $\bz_i$, we first sample $|\bz_i|$ from a distribution $Q$ and then sample a permutation of $\{1,2,\cdots, d\}$ uniformly, finally, the first $|\bz_i|$ elements in the permutation are set to 1 and the rest are set to 0.
\begin{equation}\label{eq:modified_lime}
    \bw^* = \mathop{\arg\min}_\bw \sum_{i=1}^n (f(\bz_i) - \bw^\top \bz_i)^2 + \lambda \|\bw\|^2, \bz_i \sim Q
\end{equation}  
where $Q$ is the distribution of $\bz_i$ such that 
\[
\mbp(|\bz_i| = k) = \frac{\binom{d}{k}}{A_d2^d} e^{\frac{k-d}{\sigma^2}}, \mbp(z_{i,j} = 1 | |\bz_i| = k) = \frac{k}{d}, \forall k=0,1,\cdots,d, \forall j=1,2,\cdots,d
\]
and $A_d$ is the normalization constant such that
\[
    A_d = \sum_{k=0}^d\frac{\binom{d}{k}}{2^d} e^{\frac{k-d}{\sigma^2}}    
\]
\section{proofs}
\subsection{LIME is useless with a few samples.}
\begin{theorem}\label[type]{thm:lime_weight_close_to_zero}
    Suppose we have $n$ samples $\{\bz_1, \cdots, \bz_n\}, \bz_i \sim \text{Uni}(\{0,1\}^d)$ and $\bw^*$ is the minimizer of LIME given these samples computed from \autoref{eq:lime}. 
    Then $\forall \epsilon, \delta \in (0,1)$, if $n \leq \frac{2\lambda \epsilon \mbe[\pi_i] - \sqrt{2\lambda \epsilon\mbe[\pi_i]\sqrt{d} \log \frac{1}{\delta}}}{2\sqrt{d}\mbe[\pi_i]^2}$, we have  
    $\mathbb{P}(\|\bw^*\| < \epsilon) \geq 1- \delta$.
\end{theorem}

\begin{proof}
    $\bz_i \sim \text{Uni}(\{0,1\}^d)$, $\pi(\bz) = \exp(\frac{|\bz| -d}{{\sigma}^2})$,
\[
    \bw^* = \mathop{\arg\min}_\bw \sum_i \pi(\bz_i)(f(\bz_i) - \bw^\top \bz_i)^2 + \lambda \|\bw\|^2    
\]

For $\hat{\bSigma}_n$ close to 0, we have $\|\bw^*\|< \epsilon $ with high probability.

Let $\bPi = \text{diag}(\pi(\bz_1), \cdots, \pi(\bz_n))$ and $\bZ = (\bz_1, \cdots, \bz_n), \hat{\bSigma}_n = \bZ \bPi \bZ^\top, \mathbf{F} = [f(\bz_1),\cdots, f(\bz_n)]^\top , \hat{\bGamma}_n = \bZ \bPi \mathbf{F}$, we have 
\[
    \bw^* = (\hat{\bSigma}_n + \lambda \bI )^{-1} \hat{\bGamma}_n     
\]
% Consider the case where $\lambda = 1$ which is the default of LIME. Then 

\[
\| \bw^*\| \geq \epsilon \Longleftrightarrow \|(\hat{\bSigma}_n + \lambda \bI )^{-1}\hat{\bGamma}_n\| \geq \epsilon     
\]

Since $\bz_i \in \{0,1\}^d$ and $\pi(\bz_i)> 0, \forall i$, the norm of $\hat{\bGamma}_n$ can be easily bounded 
\[
\|\hat{\bGamma}_n\| \leq \|[\sum_i \pi_i z_{i,1}, \cdots, \sum_i \pi_i z_{i,d}]^\top \| \leq \sum_i \pi_i \sqrt{d}    
\]
Then 
\[
\begin{split}
   &  \epsilon \leq   \|(\hat{\bSigma}_n +\lambda \bI )^{-1}\hat{\bGamma}_n\| \leq \|(\hat{\bSigma}_n +\lambda \bI )^{-1}\|\|\hat{\bGamma}_n\| \leq \|(\hat{\bSigma}_n +\lambda \bI)^{-1}\| \sum_i \pi_i \sqrt{d} \\ 
   & \Rightarrow \|(\hat{\bSigma}_n +\lambda \bI)^{-1}\| \geq \frac{\epsilon }{\sum_i \pi_i \sqrt{d}}
\end{split}
\]

It is easy to see that $\hat{\bSigma}_n$ is symmetric and positive definite so that its eigenvalues are all positive. We have $\lambda_{\min}(\hat{\bSigma}_n + \lambda \bI) = \lambda_{\min}(\hat{\bSigma}_n) + \lambda $. Therefore, 
\[
   \begin{split}
    &\|(\hat{\bSigma}_n + \lambda \bI)^{-1}\| = \frac{1}{\lambda_{\min}(\hat{\bSigma}_n) + \lambda }\geq \frac{\epsilon }{\sum_i \pi_i \sqrt{d}} \\ 
    & \Rightarrow \lambda \leq \lambda_{\min}(\hat{\bSigma}_n) + \lambda \leq \frac{ \sum_i \pi_i \sqrt{d}}{ \epsilon} 
   \end{split}
\]

Then we can bound $\mathbb{P}(\frac{ \sum_i \pi_i \sqrt{d}}{\epsilon}  \geq \lambda ) = \mathbb{P}(\sum_i \pi_i \geq \frac{\lambda \epsilon}{\sqrt{d}}) $ by Hoeffding inequality,
\[
        \begin{split}
             & n < \frac{2\lambda \epsilon \mbe[\pi_i] - \sqrt{2\lambda \epsilon\mbe[\pi_i]\sqrt{d} \log \frac{1}{\delta}}}{2\sqrt{d}\mbe[\pi_i]^2} \leq \frac{4\lambda \epsilon\mbe[\pi_i] /\sqrt{d}+ \log\frac{1}{\delta} - \sqrt{8\frac{\lambda \epsilon\mbe[\pi_i]}{\sqrt{d}}\log \frac{1}{\delta} + 16 \lambda^2 \epsilon^2 \mbe[\pi_i]^2/d + \log^2\frac{1}{\delta} - 16\lambda^2 \epsilon^2\mbe[\pi_i]^2/d}}{4\mbe[\pi_i]^2}\\ 
            \Longleftrightarrow& 2\mbe[\pi_i]^2 n^2 - (4\lambda \epsilon\mbe[\pi_i]/\sqrt{d} +\log\frac{1}{\delta})n + 2\lambda^2 \epsilon^2/d \geq 0 \\ 
            \Longleftrightarrow& \frac{2\mbe[\pi_i]^2(n - \frac{\lambda \epsilon}{\mbe[\pi_i]\sqrt{d}})^2}{n} \geq \log\frac{1}{\delta}\\ 
            \Longleftrightarrow &  \exp\big(-2n(\frac{\lambda \epsilon}{n\sqrt{d}} - \mbe[\pi_i])^2\big) \leq \delta \\ 
        \end{split}
    \]
\[
 \begin{split}
    \mathbb{P}(\sum_i \pi_i \geq \frac{\lambda \epsilon}{\sqrt{d}})  & =  \mathbb{P}(\frac{1}{n}\sum_i \pi_i - \mbe[{\pi_i}]\geq \frac{\lambda \epsilon}{n\sqrt{d}} - \mbe[{\pi_i}]) \\ 
    & \leq \exp(-2n( \frac{\lambda \epsilon}{n\sqrt{d}} - \mbe[{\pi_i}])^2)
 \end{split}
\]
If $n \leq \frac{2\lambda \epsilon \mbe[\pi_i] - \sqrt{2\lambda \epsilon\mbe[\pi_i]\sqrt{d} \log \frac{1}{\delta}}}{2\sqrt{d}\mbe[\pi_i]^2} $, we have 
\[
    \mathbb{P}(\sum_i \pi_i \geq \frac{\lambda \epsilon}{\sqrt{d}})  \leq \delta 
\]
and as a consequence, 
\[
\mathbb{P}(\|\bw^*\| \geq \epsilon) \leq \delta     
\]
However, is the sample complexity bound meaningful? To see why is it meaningful, we need to bound $\mathbb{E}_{\bz}[\pi(\bz)]$ 

\[
C = \mathbb{E}_{\bz}[\pi(\bz)] = \sum_{k=0}^d \frac{\tbinom{d}{k}}{2^d} e^{\frac{k-d}{{\sigma}^2}} \leq \frac{2^d - 1}{2^d} e^{-\frac{1}{{\sigma}^2}} + \frac{1}{2^d}
\]

\[
\mathbb{E}_{\bz}[\pi(\bz)] = \sum_{k=0}^d \frac{\tbinom{d}{k}}{2^d} e^{\frac{k-d}{{\sigma}^2}} \geq \frac{2^d - 1}{2^d} e^{-\frac{d}{{\sigma}^2}} + \frac{1}{2^d}
\]

And it is easy to prove that $C$ is increasing w.r.t ${\sigma}$ when ${\sigma} > 0$ is close to 0. Hence, when ${\sigma}$ becomes small, $C$ becomes small and the sample complexity bound becomes large. One implication from this is that when ${\sigma}$ is small, we need more samples to have $\|\bw^*\|\geq \epsilon$ w.p. $1-\delta$.
\end{proof}

A direct corollary from this result is that 
\[
\mathbb{P}(|w_i^* - w_j^*\| > 2\epsilon ) \leq \delta     
\]
\begin{proof}
    If $|w_i^* - w_j^*\| > 2\epsilon$, then we must have that at least one of $|w_i^*| > \epsilon$ and $|w_j^*| > \epsilon$ holds. This leads to $\|w^*\|\geq \epsilon$ which is a contradiction.
    
\end{proof}

\subsection{Concentration of $\hat{\bSigma}_n$ and $\hat{\bGamma}_n$}

Denote $\bSigma = \mathbb{E}_{\bz_1, \cdots, \bz_n}[\frac{1}{n}\hat{\bSigma}_n], \bGamma = \mathbb{E}_{\bz_1, \cdots, \bz_n}[\frac{1}{n}\hat{\bGamma}_n]$. We derive the closed form expression for $\bSigma$ in the following. 
\subsubsection{Closed Form Expression of $\mathbf{\Sigma}$}
Since $\hSigma_n = \bZ \bPi \bZ$, we have 
\[
\frac{1}{n}\hSigma_n = \begin{bmatrix}
    \frac{1}{n}\sum_i \pi_i z_{i,1}^2 &  \frac{1}{n}\sum_i \pi_i z_{i,1}z_{i,2}& \cdots &  \frac{1}{n}\sum_i \pi_i z_{i,1}z_{i,d} \\ 
    \frac{1}{n}\sum_i \pi_i z_{i,1}z_{i,2} & \frac{1}{n}\sum_i \pi_i z_{i,2}^2 & \cdots & \frac{1}{n}\sum_i \pi_i z_{i,2 }z_{i,d} \\ 
    \vdots & \vdots & \ddots & \vdots \\ 
    \sum_i \pi_i z_{i,1}z_{i,d} & \sum_i \pi_i z_{i,2}z_{i,d} & \cdots & \sum_i \pi_i z_{i,d}^2 \\ 
\end{bmatrix}
\]

Because $z_{i,j}\overset{\text{i.i.d.}}{\sim} \text{Bernoulli}(0.5, 1), \forall i, j$, the expression of $\bSigma$ can be simplified 
\[
\bSigma = \begin{bmatrix}
    \alpha_1&  \alpha_2 & \cdots & \alpha_2\\ 
    \alpha_2 & \alpha_1 & \cdots & \alpha_2 \\ 
    \vdots & \vdots & \ddots & \vdots \\ 
    \alpha_2 & \alpha_2 & \cdots & \alpha_1 \\ 
\end{bmatrix}
\] 
where 
\[
\alpha_1 = \frac{1}{n} \mathbb{E}_{\bz_i, i=1,\cdots,n}\bigg[\sum_i \pi_i z_{i,j}^2\bigg]   , 
\]
\[
    \alpha_2 =  \frac{1}{n}\mathbb{E}_{\bz_i, i=1,\cdots,n}\bigg[\sum_i \pi_i z_{i,j} z_{i, l}\bigg]  , l\neq j  
\]
The closed form expressions of $\alpha_1, \alpha_2$ are as follows:
\[
\begin{split}
\alpha_1 & =  \frac{1}{n}\mathbb{E}_{\bz_i, i=1,\cdots, n}\bigg[\sum_i \pi_i z_{i,j}^2\bigg] \\ 
& =  \frac{1}{n}\sum_i \mbe_{\bz_i}\bigg[\pi_i z_{i,j}^2\bigg] \\ 
& =  \frac{1}{n}\sum_i \sum_{k=0}^{d}e^{\frac{k-d}{\sigma^2}} \mbp(z_{i,j}=1 , |\bz_i| =k)\\
& =  \frac{1}{n}\sum_i \sum_{k=1}^{d}e^{\frac{k-d}{\sigma^2}} \mbp(z_{i,j}=1 ||\bz_i| =k)\mbp(|\bz_i| = k)\\
& =  \frac{1}{n}\sum_i \sum_{k=1}^{d}e^{\frac{k-d}{\sigma^2}}  \frac{k}{d}\frac{\binom{d}{k}}{2^d}\\
& =  \sum_{k=0}^{d-1}e^{\frac{k-d}{\sigma^2}} \frac{\binom{d-1}{k}}{2^d} \\
\end{split}
\]

\[
\begin{split}
\alpha_2 & =  \frac{1}{n}\mathbb{E}_{\bz_i, i=1,\cdots, n}\bigg[\sum_i \pi_i z_{i,j}z_{i,l}\bigg] \\ 
& =  \frac{1}{n}\sum_i \mbe_{\bz_i}\bigg[\pi_i z_{i,j}z_{i,l}\bigg] \\ 
& =  \frac{1}{n}\sum_i \sum_{k=0}^{d}e^{\frac{k-d}{\sigma^2}} \mbp(z_{i,j}=1, z_{i,l}=1 , |\bz_i| =k)\\
& =  \frac{1}{n}\sum_i \sum_{k=2}^{d}e^{\frac{k-d}{\sigma^2}} \mbp(z_{i,j}=1, z_{i,l}=1||\bz_i| =k)\mbp(|\bz_i| = k)\\
& =  \frac{1}{n}\sum_i \sum_{k=2}^{d}e^{\frac{k-d}{\sigma^2}}  \frac{k(k-1)}{d(d-1)}\frac{\binom{d}{k}}{2^d}\\
& =  \sum_{k=0}^{d-2}e^{\frac{k-d}{\sigma^2}} \frac{\binom{d-2}{k}}{2^d} \\
\end{split}
\]

To explore further, we can bound $\alpha_1, \alpha_2$ as stated in the following Proposition 

\begin{proposition}
    $\alpha_1, \alpha_2$ are both lower and upper bounded.
    \[
        \frac{1}{2}\exp\big(-\frac{d + 1}{2\sigma^2}\big)\leq \alpha_1 \leq \frac{e^{-\frac{1}{\sigma^2}}}{2},  
    \]
    \[
        \frac{1}{4}\exp\big(-\frac{d + 2}{2\sigma^2}\big)\leq \alpha_2 \leq \frac{e^{-\frac{2}{\sigma^2}}}{4}    
    \]
\end{proposition}
\begin{proof}
    Because $\sum_k \binom{d-1}{k} = 2^{d-1}$, and thus we can view $\binom{d-1}{k}/ 2^{d-1}$ as the weight for $e^{\frac{k-d}{\sigma^2}}$. And then we are allowed to use Jensen's inequality to lower bound $\alpha_1$ since $e^{\frac{x}{\sigma^2}}$ is a convex function w.r.t. $x$. 

    \[
        \alpha_1 = \sum_{k=0}^{d-1}e^{\frac{k-d}{\sigma^2}} \frac{\binom{d-1}{k}}{2^d} \leq \sum_{k=0}^{d-1}e^{\frac{d-1-d}{\sigma^2}} \frac{\binom{d-1}{k}}{2^d} = \frac{e^{-\frac{1}{\sigma^2}}}{2}
    \]
    \[
    \begin{split}
        \alpha_1 =&  \sum_{k=0}^{d-1}e^{\frac{k-d}{\sigma^2}} \frac{\binom{d-1}{k}}{2^d} \\ 
        \geq & \frac{e^{-\frac{d}{\sigma^2}}}{2}\exp\big(\sum_k \frac{k\binom{d-1}{k}}{2^{d-1}\sigma^2}\big)\\ 
        = & \frac{e^{-\frac{d}{\sigma^2}}}{2}\exp\big(\sum_k \frac{(d-1)\binom{d-2}{k-1}}{2^{d-1}\sigma^2}\big)\\ 
        = & \frac{e^{-\frac{d}{\sigma^2}}}{2}\exp\big(\frac{d-1}{2\sigma^2}\big)\\ 
         = & \frac{1}{2}\exp\big(-\frac{d + 1}{2\sigma^2}\big)
    \end{split}
    \]
    The second equality above holds by the fact 
    \[
    k\binom{d-1}{k} = k\frac{(d-1)!}{k!(d-1-k)!} = \frac{(d-1)!}{(k-1)!(d-1-k)!} = (d-1)\frac{(d-2)!}{(k-1)!(d-1-k)!} = (d-1) \binom{d-2}{k-1}
    \]

    We can bound $\alpha_2$ similarly. 

    \[
        \alpha_2 = \sum_{k=0}^{d-2}e^{\frac{k-d}{\sigma^2}} \frac{\binom{d-2}{k}}{2^d} \leq \sum_{k=0}^{d-2}e^{\frac{d-2-d}{\sigma^2}} \frac{\binom{d-2}{k}}{2^d} = \frac{e^{-\frac{2}{\sigma^2}}}{4}
    \]
    \[
        \begin{split}
            \alpha_2 =&  \sum_{k=0}^{d-2}e^{\frac{k-d}{\sigma^2}} \frac{\binom{d-2}{k}}{2^d} \\ 
            \geq & \frac{e^{-\frac{d}{\sigma^2}}}{4}\exp\big(\sum_k \frac{k\binom{d-2}{k}}{2^{d-2}\sigma^2}\big)\\ 
            = & \frac{e^{-\frac{d}{\sigma^2}}}{4}\exp\big(\sum_k \frac{(d-2)\binom{d-3}{k-1}}{2^{d-2}\sigma^2}\big)\\ 
            = & \frac{e^{-\frac{d}{\sigma^2}}}{4}\exp\big(\frac{d-2}{2\sigma^2}\big)\\ 
             = & \frac{1}{4}\exp\big(-\frac{d + 2}{2\sigma^2}\big)
        \end{split}
        \]

\end{proof}
\subsubsection{Concentration of $\alpha_1$ and $\alpha_2$}
\begin{proposition}
    For any $t > 0$, 
    \[
    \mbp(|\hat{\alpha}_1 - \alpha_1 | > t) < 2 e^{-2nt^2}    
    \]
    \[
    \mbp(|\hat{\alpha}_2 - \alpha_2 | > t) < 2 e^{-2nt^2}    
    \]
\end{proposition}
\begin{proof}
    $\hat{\alpha}_1$ is bounded:
\[
    0 \leq  \hat{\alpha}_1 = \frac{1}{n}\sum_i \pi_i z_{i,1} \leq \frac{1}{n}\sum_{i} z_{i,1} \leq 1   
\]
\[
    0 \leq  \hat{\alpha}_2 = \frac{1}{n}\sum_i \pi_i z_{i,1}z_{i,2} \leq \frac{1}{n}\sum_{i} z_{i,1}z_{i,2} \leq 1   
\]
    Then the conclusion follows directly from Hoeffding inequality.

\end{proof}


Since $\bw^* = (\hat{\bSigma}_n + \frac{1}{n}\lambda \bI)^{-1}\hat{\bGamma}_n$, when $n$ is large the effect of $\frac{1}{n}\lambda \bI$ may be ignored. We proceed to see when this would happen. 

It is easy to see that $\hat{\bSigma}_n$ is positive definite and $\hat{\alpha}_1, \hat{\alpha}_2$ are non-negative.  Only the diagonal terms are affected. So we only consider $\hat{y}$ and ${\lambda}$, where $\hat{y} = \frac{1}{n}\sum_i \pi_i \sum_j z_{i,j}/d$. 

We have the following Theoerem.

\begin{theorem}\label[type]{thm:concentrate_orig}
Let $\alpha_0 = \mbe[y_i]$.    For any $t >0, \delta \in (0,1)$, if $n \leq \frac{2\lambda t \alpha_0 - \sqrt{2\lambda t\alpha_0 \log \frac{1}{\delta}}}{2\alpha_0^2}$, we have 
    \[
    \mbp(\hat{y} > \frac{\lambda }{n}t) \leq     \delta 
    \]
\end{theorem}

\begin{proof}
    We first reformulate the expression of $\hat{y}$, let $y_i =  \pi_i \sum_j z_{i,j}/d  = \pi_i | \bz_i|/d$, then $\hat{y} = \frac{1}{n} \sum_i y_i$, 
    \[
    \mbp(y_i = k/d) = \frac{\binom{d}{k}}{2^d} e^{\frac{k-d}{\sigma^2}},    
    \]

    \[
        \mbe[y_i] = \sum_{k=0}^{d}\frac{k}{d} \frac{\binom{d}{k}}{2^d} e^{\frac{k-d}{\sigma^2}   }  =\sum_{k=0}^{d}\frac{\binom{d-1}{k-1}}{2^d} e^{\frac{k-d}{\sigma^2}   } = \alpha_1 e^{\frac{1}{\sigma^2}} = \alpha_0, \mbe[\hat{y}] = \alpha_0
    \]

    For $n \leq \frac{2\lambda t \alpha_0 - \sqrt{2\lambda t\alpha_0 \log \frac{1}{\delta}}}{2\alpha_0^2}\leq \frac{\lambda  t}{\alpha_0}$
    \[
        \hat{y} > \frac{\lambda }{n}t \Longleftrightarrow \hat{y} - \alpha_0 > \frac{\lambda t}{n} - \alpha_0 > 0
    \]
Since $0\leq y_i \leq 1$, thus by Hoeffding inequality, we have 
    \[
    \begin{split}
        \mbp( \hat{y} - \alpha_0 > \frac{\lambda t}{n} - \alpha_0)   & \leq \exp\big(-2n(\frac{\lambda t}{n} - \alpha_0)^2\big)\\ 
    \end{split}
    \]
    Because
    \[
        \begin{split}
             & n < \frac{2\lambda t \alpha_0 - \sqrt{2\lambda t\alpha_0 \log \frac{1}{\delta}}}{2\alpha_0^2} \leq \frac{4\lambda t \alpha_0 + \log\frac{1}{\delta} - \sqrt{8\lambda t\alpha_0 \log \frac{1}{\delta} + 16 \lambda^2 t^2 \alpha_0^2 + \log^2\frac{1}{\delta} - 16\lambda^2 t^2\alpha_0^2}}{4\alpha_0^2}\\ 
            \Longleftrightarrow& 2\alpha_0^2 n^2 - (4\lambda t\alpha_0 +\log\frac{1}{\delta})n + 2\lambda^2 t^2 \geq 0 \\ 
            \Longleftrightarrow& \frac{2\alpha_0^2(n - \frac{\lambda t}{\alpha_0})^2}{n} \geq \log\frac{1}{\delta}\\ 
            \Longleftrightarrow &  \exp\big(-2n(\frac{\lambda t}{n} - \alpha_0)^2\big) \leq \delta \\ 
        \end{split}
    \]
There are many implication from this result:
\begin{itemize}
    \item If we only have limited data, the penalty term may dominate the solution, as $\hat{\alpha}_1 \leq \frac{\lambda t}{n}$ with probability of at least $1 - \delta $
    \item Since the sample complexity bound is of order $O(\frac{1}{\alpha_0})$, when the kernel width $\sigma$ becomes smaller, i.e., putting more weight on similar samples, the number of samples required for the sum-of-square-error term to take into work increases in order $O(e^{\frac{d-1}{2\sigma^2}})$ as $\alpha_1$ is lower bounded by $\frac{1}{2}\exp(-\frac{d+1}{2\sigma^2})$
    \item When the parameter $\lambda$ in the ridge penalty term becomes large, we need more data to make $\hat{\alpha}_1$ take control, which is very intuitive.
\end{itemize}
\end{proof}


\subsection{Concentration of Improved Sampling Algorithm}

Denote $w_i = |\bz_i|/d, \hat{w} = \frac{1}{n}\sum_i w_i $, then we have 
\begin{theorem}\label[type]{thm:concentrate_reformulate}
    Let $\gamma = \mbe[w_i]$. For any $t >0, \delta \in (0,1)$, if $n \leq \frac{2\lambda t \gamma - \sqrt{2\lambda t\gamma \log \frac{1}{\delta}}}{2\gamma^2}$, we have 
    \[
    \mbp(\hat{w} > \frac{\lambda }{n}t) \leq     \delta 
    \]
\end{theorem}

\begin{proof}
    Under our new sampling distribution, the distribution of $w_i$ is as follows:
    \[
    \mbp(w_i = k/d) = \frac{1}{A_d}\frac{\binom{d}{k}}{2^d} e^{\frac{k-d}{\sigma^2}   },    A_d = \sum_k \frac{\binom{d}{k}}{2^d} e^{\frac{k-d}{\sigma^2}}
    \]

    \[
        \mbe[w_i] = \frac{1}{A_d}\sum_{k=0}^{d}\frac{k}{d} \frac{\binom{d}{k}}{2^d} e^{\frac{k-d}{\sigma^2}   }  = \frac{1}{A_d} \sum_{k=0}^{d}\frac{\binom{d-1}{k-1}}{2^d} e^{\frac{k-d}{\sigma^2}   } = \frac{A_{d-1}}{2A_d} = \gamma, \mbe[\hat{w}] = \gamma
    \]

    For $n \leq \frac{2\lambda t \gamma - \sqrt{2\lambda t\gamma \log \frac{1}{\delta}}}{2\bGamma^2}\leq \frac{\lambda  t}{\gamma}$
    \[
        \hat{w} > \frac{\lambda }{n}t \Longleftrightarrow \hat{w} - \gamma > \frac{\lambda t}{n} - \gamma > 0
    \]
Since $0\leq y_i \leq 1$, thus by Hoeffding inequality, we have 
    \[
    \begin{split}
        \mbp( \hat{w} - \gamma > \frac{\lambda t}{n} - \gamma)   & \leq \exp\big(-2n(\frac{\lambda t}{n} - \gamma)^2\big)\\ 
    \end{split}
    \]
    Because
    \[
        \begin{split}
             & n < \frac{2\lambda t \gamma - \sqrt{2\lambda t\gamma \log \frac{1}{\delta}}}{2\gamma^2} \leq \frac{4\lambda t \gamma + \log\frac{1}{\delta} - \sqrt{8\lambda t\gamma \log \frac{1}{\delta} + 16 \lambda^2 t^2 \gamma^2 + \log^2\frac{1}{\delta} - 16\lambda^2 t^2\gamma^2}}{4\gamma^2}\\ 
            \Longleftrightarrow& 2\gamma^2 n^2 - (4\lambda t\gamma +\log\frac{1}{\delta})n + 2\lambda^2 t^2 \geq 0 \\ 
            \Longleftrightarrow& \frac{2\gamma^2(n - \frac{\lambda t}{\gamma})^2}{n} \geq \log\frac{1}{\delta}\\ 
            \Longleftrightarrow &  \exp\big(-2n(\frac{\lambda t}{n} - \gamma)^2\big) \leq \delta \\ 
        \end{split}
    \]

\end{proof}

Note that the sample complexity bound has the same form as that in \autoref{thm:concentrate_orig} but with $\gamma$ in stead of $\alpha_0$. This small change actually makes huge difference on the sample complexity bounds. This is due to the fact that $\gamma$ is lower bounded by a positive number that is independent of $e^{-\frac{1}{\sigma^2}}$. When $\sigma$ is small, the sample complexity boundd doe not grow exponentially as it is in the original sampling algorithm. The bound on $\gamma$ is stated in the next Proposition. 

\begin{proposition}
    $\frac{1}{4} \leq \gamma \leq \frac{1}{2}$
\end{proposition}
\begin{proof}
    \[
    \begin{split}
        \gamma = &  \frac{1}{2A_d}\sum_{k=0}^{d}\frac{k}{d} \frac{\binom{d}{k}}{2^d} e^{\frac{k-d}{\sigma^2}} \leq \frac{1}{2A_d}\sum_{k=0}^{d}\frac{d}{d} \frac{\binom{d}{k}}{2^d} e^{\frac{k-d}{\sigma^2}} = \frac{A_d}{2A_d} = \frac{1}{2} \\ 
    \end{split}
    \]
    Let 
    \[
    \rho =     \frac{1}{2A_d}\sum_{k=0}^{d}\frac{d-k}{d} \frac{\binom{d}{k}}{2^d} e^{\frac{k-d}{\sigma^2}} 
    \]
    then we have 
    \[
    \gamma + \rho = \frac{1}{2A_d}\sum_{k=0}^{d}\frac{d}{d} \frac{\binom{d}{k}}{2^d} e^{\frac{k-d}{\sigma^2}}  = 1
    \]
    However, if $d = 2m, m \in \mathbb{N}_+$, we have 
    % \[
    %     \rho = \frac{1}{A_d}\sum_{k=0}^{d}\frac{k}{d} \frac{\binom{d}{d-k}}{2^d} e^{-\frac{k}{\sigma^2}}  =  \frac{1}{A_d}\sum_{k=0}^{d}\frac{k}{d} \frac{\binom{d}{k}}{2^d} e^{-\frac{k}{\sigma^2}}
    % \]
    % Then 
    \[
    \begin{split}
        \gamma - \rho & =  \frac{1}{2A_d}\sum_{k=0}^{d}\frac{(2k-d)}{d} \frac{\binom{d}{k}}{2^d} e^{\frac{k-d}{\sigma^2}} \\ 
        & = \frac{1}{2A_d}\sum_{k=0}^{m} \bigg[\frac{(2k-d)}{d} \frac{\binom{d}{k}}{2^d} e^{\frac{k-d}{\sigma^2}} + \frac{(2(d-k)-d)}{d} \frac{\binom{d}{k}}{2^d} e^{\frac{d-k-d}{\sigma^2}}\bigg] \\ 
        & =  \frac{1}{2A_d}\sum_{k=0}^{m} \bigg[\frac{(2k-d)}{d} \frac{\binom{d}{k}}{2^d} e^{\frac{k-d}{\sigma^2}} + \frac{(d-2k)}{d} \frac{\binom{d}{k}}{2^d} e^{-\frac{k}{\sigma^2}}\bigg] \\ 
        & =  \frac{1}{2A_d}\sum_{k=0}^{m} \bigg[\frac{(d-2k)}{d} \frac{\binom{d}{k}}{2^d} \big(e^{-\frac{k}{\sigma^2}} - e^{\frac{k-d}{\sigma^2}}\big) \bigg] \\
        & \geq 0 
    \end{split}
    \]
    The last inequality is due to 
    \[
        e^{-\frac{k}{\sigma^2}} - e^{\frac{k-d}{\sigma^2}} = e^{-\frac{k}{\sigma^2}}(1 - e^{\frac{2k-d}{\sigma^2}}) \geq 0, \forall k=0, \cdots, m
    \]
    For $d$ that is odd, we can leave the $\frac{d+1}{2} $th term in $\gamma - \rho$ unchanged and pair the rest terms. We can still get $\gamma - \rho \geq 0$. 

    Therefore, $\gamma \geq \rho$ and 
    \[
        \frac{1}{2} = \gamma + \rho \leq \gamma + \gamma \Longrightarrow \gamma\geq \frac{1}{4}    
    \]
\end{proof}

Therefore, unlike $\alpha_0$, $\gamma$ is lower bounded by a constant that is independent of $\sigma$ which ensures a better sample complexity shown in \autoref{thm:concentrate_reformulate}. 

In the original formulation, when kernel width $\sigma$ is small, \autoref{thm:concentrate_orig} shows that we need a lot of data to make the sum-of-square-error term be comparable with the regularization term. And the number of data required increases exponentially fast w.r.t $\frac{d}{2\sigma^2}$. if we do not have many data, the solution return by LIME may be useless and close to a vector of 0 as shown in \autoref{thm:lime_weight_close_to_zero}. While in the modified formulation, when $\sigma$ is small, $\gamma$ is much larger than $\alpha_0$ which allows our algorithm to return more meaningful and stable solutions.


\section{Proof of Faithfulness}
\[
\sigma_0 = (\alpha_1 - \alpha_2)(\alpha_1 + (d-1)\alpha_2), \sigma_1 = \alpha_1 + (d-1)\alpha_2, \sigma_2 =-\alpha_2    
\]
\begin{lemma}
    When $\sigma \to \infty$, 
    \[
    \alpha_1 \to \frac{1}{2}, \alpha_2 \to \frac{1}{4}, \alpha_1 - \alpha_2 \to \frac{1}{4}, A_d \to 1, \gamma \to \frac{1}{2}    
    \]

    When $\sigma \to 0$, 
    \[
    \alpha_1 = O(e^{-\frac{1}{\sigma^2}}), \alpha_2  = O(e^{-\frac{2}{\sigma^2}}), \frac{\alpha_2}{(\alpha_1 - \alpha_2)(\alpha_1 + (d-1)\alpha_2)} \to 1, A_d \to \frac{1}{2^d}, \gamma \to \frac{1}{4}
    \]
\end{lemma}
\begin{proof}
    \[
    \begin{split}
        \alpha_1 & =  \sum_{k=0}^{d-1}e^{\frac{k-d}{\sigma^2}} \frac{\binom{d-1}{k}}{2^d} \to \sum_{k=0}^{d-1}\frac{\binom{d-1}{k}}{2^d} = \frac{1}{2}\\
    \end{split}
    \]

    \[
    \begin{split}
        \alpha_2& = \sum_{k=0}^{d-2}e^{\frac{k-d}{\sigma^2}} \frac{\binom{d-2}{k}}{2^d}  \to  \sum_{k=0}^{d-2} \frac{\binom{d-2}{k}}{2^d} = \frac{1}{4}\\    \end{split}
    \]
    \[
    A_d =   \sum_{k=0}^{d}e^{\frac{k-d}{\sigma^2}} \frac{\binom{d}{k}}{2^d}  \to  \sum_{k=0}^{d} \frac{\binom{d}{k}}{2^d} = 1
    \]
    Similarly, $A_{d-1} \to 1$, and thus 
    \[
    \gamma = \frac{A_{d-1}}{2A_d} \to \frac{1}{2}    
    \]

    \[
    \frac{\sigma_2}{\sigma_0} = - \frac{\alpha_2}{(\alpha_1 - \alpha_2)(\alpha_1 + (d-1)\alpha_2)} \to \frac{4}{d + 1}     
    \]
    \[
    \frac{\sigma_1 - \sigma_2}{\sigma_0} = \frac{1}{\alpha_1 - \alpha_2} \to 4    
    \]
\end{proof}
Infidelity is defined as:
\[
p(x)_i = f(x) - f(x\odot e_{-i}), e_{-i} = \mathbf{1} - e_i
\]
\[
I(\phi, p) = {\|\phi - p\|}
\]

\begin{theorem}
    we can prove 
\end{theorem}
\begin{proof}
    \[
    \phi(\bx) = \frac{1}{\sigma_0}\big[\sigma_2 \mathbb{E}[|\bz|f(\bz)] \mathbf{1} + (\sigma_1 - \sigma_2)\Gamma \big]
    \]

    \[
    \begin{split}
        (\phi_i(\bx) - p_i(\bx))^2 & =  ( \frac{1}{\sigma_0}\big[\sigma_2 \mathbb{E}[|\bz|f(\bz)] + (\sigma_1 - \sigma_2)\Gamma_i \big] - (f(\bone) - f(e_{-i})))^2 \\
        & = ((\frac{\sigma_2}{\sigma_0}\mathbb{E}[|\bz|f(\bz)] + f(e_{-i})) + (\frac{\sigma_1 - \sigma_2}{\sigma_0}\Gamma_i - f(\bone)))^2 \\
    \end{split}
    \]
    Denote $M = \frac{\sigma_2}{\sigma_0}\mathbb{E}[|\bz|f(\bz)]$ and $T_i = \frac{\sigma_1 - \sigma_2}{\sigma_0}\Gamma_i$, then we have
    \[
    \begin{split}
        \|\phi(\bx) - p(\bx)\|^2 & = \sum_{i=1}^d  (\phi_i(\bx) - p_i(\bx))^2 = \sum_{i=1}^d \bigg[(M + f(e_{-i})) + (T_i - f(\bone))\bigg]^2 \\ 
& =  \sum_{i=1}^d \bigg[(M + f(e_{-i}))^2 + (T_i - f(\bone))^2\bigg]  + 2\sum_{i=1}^d (M + f(e_{-i}))(T_i - f(\bone)) \\
        & = A + B + C\\
    \end{split}
    \]
    where 
    \[
        A = \sum_{i=1}^d (M + f(e_{-i}))^2, B = \sum_{i=1}^d (T_i - f(\bone))^2, C = 2\sum_{i=1}^d (M + f(e_{-i}))(T_i - f(\bone)) 
    \]
    \[
    \begin{split}
        A & = \sum_{i=1}^d (M + f(e_{-i}))^2 \\ 
         & = \sum_{i=1}^d (M - \frac{\sigma_2}{\sigma_0}\mbe[|\bz|] f(e_{-i}) + \frac{\sigma_2}{\sigma_0}\mbe[|\bz|] f(e_{-i}) + f(e_{-i}))^2\\ 
         & = \sum_{i=1}^d (M - \frac{\sigma_2}{\sigma_0}\mbe[|\bz|] f(e_{-i}))^2 + \sum_{i=1}^d  (f(e_{-i}) + \frac{\sigma_2}{\sigma_0}\mbe[|\bz|] f(e_{-i}))^2 + 2\sum_{i=1}^d (M - \frac{\sigma_2}{\sigma_0}\mbe[|\bz|] f(e_{-i})) (f(e_{-i}) + \frac{\sigma_2}{\sigma_0}\mbe[|\bz|] f(e_{-i}))\\
         & = A_1 + A_2 + A_3 \\ 
    \end{split}
    \]
    where 
    \[
    \begin{split}
        A_1 = & \sum_{i=1}^d (M - \frac{\sigma_2}{\sigma_0}\mbe[|\bz|] f(e_{-i}))^2 \\ 
        A_2 = & \sum_{i=1}^d  (f(e_{-i})+ \frac{\sigma_2}{\sigma_0}\mbe[|\bz|] f(e_{-i}))^2  = \sum_{i=1}^d  f(e_{-i})^2(1 + \frac{\sigma_2}{\sigma_0}\mbe[|\bz|])^2\\ 
        A_3 = & 2\sum_{i=1}^d (M - \frac{\sigma_2}{\sigma_0}\mbe[|\bz|] f(e_{-i})) (f(e_{-i}) + \frac{\sigma_2}{\sigma_0}\mbe[|\bz|] f(e_{-i})) \\ 
    \end{split}
    \]

   
    \[
    \sigma\to \infty, \alpha_2 \to \frac{1}{4}, \alpha_1\to\frac{1}{2}, \gamma \to \frac{1}{4}    
    \]
    Thus, 
    \[
        \frac{\sigma_2}{\sigma_0}\mbe[|\bz|] = -\frac{\alpha_2}{(\alpha_1 - \alpha_2)(\alpha_1 + (d-1) \alpha_2}\gamma d \to -\frac{2d}{d+1}, \sigma\to \infty 
     \]
     \[
     A_2 \to \frac{(d-1)^2}{(d+1)^2}\sum_{i=1}^d f^2(e_{-i})
     \]
     Since when $\sigma\to \infty$ the distribution of $\bz$ tends to uniform distribution, we have 
     \[
     \begin{split}
        A_1 & = \sum_{i=1}^d (M - \frac{\sigma_2}{\sigma_0}\mbe[|\bz|] f(e_{-i}))^2 \\ 
        & = \sum_{i=1}^d (\frac{\sigma_2}{\sigma_0}\mbe[|\bz|] f(\hat{\xi}) - \frac{\sigma_2}{\sigma_0}\mbe[|\bz|] f(e_{-i}))^2 \\ 
        & \to  \sum_{i=1}^d (-\frac{2d}{d+1} f(\xi) +\frac{2d}{d+1} f(e_{-i}))^2  = \sum_{i=1}^d (\frac{2d}{d+1})^2(f(\xi) -f(e_{-i}))^2 \\ 
     \end{split}
     \]

     when $\sigma$ is very large, $\mathbb{E}[|\bz|f(\bz)] < f(e_{-i}), \forall i=1,\cdots,d$
     \[
     A_3 =    2\sum_{i=1}^d (M - \frac{\sigma_2}{\sigma_0}\mbe[|\bz|] f(e_{-i})) (f(e_{-i}) + \frac{\sigma_2}{\sigma_0}\mbe[|\bz|] f(e_{-i})) > 0
     \]
     Hence, 
     \[
    \lim_{\sigma \to \infty} A \geq \lim_{\sigma\to\infty} A_1 + \lim_{\sigma\to\infty} A_2 
     \]



\section{The Exact Expression of $\*w$: Linear Case}
Assume there is D pixels in an image, and we have $f(\*x) = \sum_{i=1}^D \lambda_i x_i$ is a linear model. We calculate $\*w$ for $\*x$ in this linear case. When computing explanations, in the implementation of LIME, samples' output is first normalized by subtracting their mean. Therefore, we first define $g(\*x\odot \*z) = f(\*x\odot \*z) - \mathbb{E}_{\*z^\prime\sim P_{\*x}}[f(\*x \odot \*z^\prime)], \forall z \sim P_{\*x}$, i.e., for a sample we generated around $\*x$, we subtract its model output by the output mean over the entire distribution. 

Note, in this case, we have 
\[
w_i = \frac{1}{\sigma_0}\big[\sigma_2\mathbb{E}[|\*z| g(\*z)] + (\sigma_1 - \sigma_2) \mathbb{E}[z_i g(\*z)]\big], \forall i =1,\cdots, d
\]
\[
\sigma_0 = (\alpha_1 - \alpha_2)(\alpha_1 + (d-1)\alpha_2), \sigma_1 = \alpha_1 +(d-2)\alpha_2, \sigma_2 = -\alpha_2
\]
\[
\alpha_1 = \mathbb{E}[z_i] = \frac{1}{1 + e^{-\frac{1}{\sigma^2}}}, \alpha_2 = \mathbb{E}[z_iz_j] = \frac{1}{(1 + e^{-\frac{1}{\sigma^2}})^2}, \alpha_1 - \alpha_2 = \frac{e^{-\frac{1}{\sigma^2}}}{(1 + e^{-\frac{1}{\sigma^2}})^2}
\]
\[
\frac{\sigma_1 - \sigma_2}{\sigma_0} = \frac{1}{\alpha_1-\alpha_2} = \frac{(1 + e^{-\frac{1}{\sigma^2}})^2}{e^{-\frac{1}{\sigma^2}}}
\]
\[
\frac{\sigma_2}{\sigma_0} = -\frac{\alpha_2}{(\alpha_1 - \alpha_2)(\alpha_1 + (d-1)\alpha_2)} = -\frac{e^{\frac{1}{\sigma^2}}}{\frac{1}{1 + e^{-\frac{1}{\sigma^2}}} + \frac{d-1}{(1 + e^{-\frac{1}{\sigma^2}})^2}} = -\frac{(1 + e^{\frac{1}{\sigma^2}})^2}{1 + de^{\frac{1}{\sigma^2}}}
\]
Since the expression of $\*w$ is linear w.r.t. $f$, we can first consider $f(\*x) = x_j$. Assume $x_j$ is in superpixel $j$, then we have 
\[
\begin{split}
    \mathbb{E}_{\*z^\prime\sim P_{\*x}}[f(\*x \odot \*z^\prime)] & = \sum_{k=0}^d \mbp(|\*z| = k, z_j = 1) x_i + \sum_{k=0}^d \mbp(|\*z| = k, z_j = 0) (x_i - r) \\ 
    & = \sum_{k=0}^d \frac{\binom{d-1}{k-1} e^{\frac{k}{\sigma^2}}}{A_d} x_i + \sum_{k=0}^d \frac{\binom{d-1}{k} e^{\frac{k}{\sigma^2}}}{A_d} (x_i - r) \\ 
    & = \frac{e^{\frac{1}{\sigma^2}}}{1 + e^{\frac{1}{\sigma^2}}} x_i + \frac{1}{1 + e^{\frac{1}{\sigma^2}}} (x_i -r) \\ 
    & = x_i - \frac{1}{1 + e^{\frac{1}{\sigma^2}}} r
\end{split}
\]

$g(\*z) = x_i - (x_i -  \frac{1}{1 + e^{\frac{1}{\sigma^2}}} r) =  \frac{1}{1 + e^{\frac{1}{\sigma^2}}} r$ if $z_j = 1$, otherwise, $g(\*z) = 0 - (x_i -  \frac{1}{1 + e^{\frac{1}{\sigma^2}}} r) = \frac{1}{1 + e^{\frac{1}{\sigma^2}}} r - x_i$
\[
\begin{split}
    \mbe[|\*z| g(\*z)] &= \sum_{k=0}^d \mbp(|\*z| = k) k g(\*z)\\
    & = \sum_{k=0}^d \mbp(|\*z| =k, z_j = 1) k g(\*z) + \sum_{k=0}^d \mbp(|\*z| =k, z_j = 0) k g(\*z) \\ 
    & = \sum_{k=0}^d \frac{\binom{d-1}{k-1} e^{\frac{k}{\sigma^2}}}{A_d} k\frac{1}{1 + e^{\frac{1}{\sigma^2}}} r + \sum_{k=0}^d \frac{\binom{d-1}{k} e^{\frac{k}{\sigma^2}}}{A_d} k (\frac{1}{1 + e^{\frac{1}{\sigma^2}}} r - x_i) \\ 
    & = \frac{(d-1) e^{\frac{2}{\sigma^2}}}{(1 + e^{\frac{1}{\sigma^2}})^3}r + \frac{e^{\frac{1}{\sigma^2 }}}{(1 + e^{\frac{1}{\sigma^2}})^2}r + \frac{(d-1) e^{\frac{1}{\sigma^2}}}{(1 + e^{\frac{1}{\sigma^2}})^2}(\frac{1}{1 + e^{\frac{1}{\sigma^2}}} r - x_i) \\ 
    & = \frac{d(1+e^{\frac{1}{\sigma^2}})}{(1 + e^{\frac{1}{\sigma^2}})^3} r - \frac{(d-1) e^{\frac{1}{\sigma^2}}}{(1 + e^{\frac{1}{\sigma^2}})^2} x_i\\ 
    & = \frac{d}{(1 + e^{\frac{1}{\sigma^2}})^2} r - \frac{(d-1) e^{\frac{1}{\sigma^2}}}{(1 + e^{\frac{1}{\sigma^2}})^2} x_i\\ 
\end{split}
\]
\[
\frac{\sigma_2}{\sigma_0} \mbe[|\*z| g(\*z)] =- \frac{dr}{1 + de^{\frac{1}{\sigma^2}}} + \frac{(d-1) e^{\frac{1}{\sigma^2}}}{1 + de^{\frac{1}{\sigma^2}}}x_i
\]

For $l = j$, we have 
\[
\begin{split}
    \mbe[z_l g(\*z)] & = \sum_{k=0}^d \mbp(|\*z| = k, z_l = 1) \frac{1}{1 + e^{\frac{1}{\sigma^2}}} r \\ 
    & = \sum_{k=0}^d \frac{\binom{d-1}{k-1}e^{\frac{k}{\sigma^2}}}{A_d} \frac{1}{1 + e^{\frac{1}{\sigma^2}}} r \\ 
    & = \frac{e^{\frac{1}{\sigma^2}}}{(1 + e^{\frac{1}{\sigma^2}})^2} r
\end{split}
\]
\[
\frac{\sigma_1 - \sigma_2}{\sigma_0}\mbe[z_l g(\*z)] = r
\]
For $l\neq j$, we have 
\[
\begin{split}
    \mbe[z_l g(\*z)] & = \sum_{k=0}^d \mbp(|\*z| = k, z_l = 1, z_j=1) \frac{1}{1 + e^{\frac{1}{\sigma^2}}} r + \sum_{k=0}^d \mbp(|\*z| = k, z_l = 1, z_j = 0) \bigg(\frac{1}{1 + e^{\frac{1}{\sigma^2}}} r - x_i\bigg) \\ 
    & = \sum_{k=0}^d \frac{\binom{d-2}{k-2}e^{\frac{k}{\sigma^2}}}{A_d} \frac{1}{1 + e^{\frac{1}{\sigma^2}}} r  + \sum_{k=0}^d \frac{\binom{d-2}{k-1}e^{\frac{k}{\sigma^2}}}{A_d} \bigg(\frac{1}{1 + e^{\frac{1}{\sigma^2}}} r - x_i\bigg) \\ 
    & = \frac{e^{\frac{2}{\sigma^2}}}{(1+e^{\frac{1}{\sigma^2}})^3} r + \frac{e^{\frac{1}{\sigma^2}}}{(1+ e^{\frac{1}{\sigma^2}})^2} \bigg(\frac{1}{1 + e^{\frac{1}{\sigma^2}}} r - x_i\bigg) \\ 
    & = \frac{e^{\frac{1}{\sigma^2}}}{(1+e^{\frac{1}{\sigma^2}})^2} r - \frac{e^{\frac{1}{\sigma^2}}}{(1+ e^{\frac{1}{\sigma^2}})^2} x_i 
\end{split}
\]
\[
\frac{\sigma_1 - \sigma_2}{\sigma_0}\mbe[z_l g(\*z)] = r - x_i
\]



We follow notations from . In our case, 
\[
\alpha_0 = 1, \alpha_1 = \mathbb{E}[z_i] = \frac{1}{1 + e^{-\frac{1}{\sigma^2}}}, \alpha_2 = \mathbb{E}[z_iz_j] = \frac{1}{(1 + e^{-\frac{1}{\sigma^2}})^2} = \alpha_1^2, \alpha_1 - \alpha_2 = \frac{e^{-\frac{1}{\sigma^2}}}{(1 + e^{-\frac{1}{\sigma^2}})^2}
\]
\[
\sigma_0 = (d-1)\alpha_2 + \alpha_1 = \frac{d + e^{-\frac{1}{\sigma^2}}}{(1 + e^{-\frac{1}{\sigma^2}})^2}
\]
\[
\sigma_1 = -\alpha_1 = - \frac{1}{1 + e^{-\frac{1}{\sigma^2}}}
\]
\[
\sigma_2 = \frac{(d-2)\alpha_0\alpha_2 - (d-1)\alpha_1^2 + \alpha_0\alpha_1}{\alpha_1 - \alpha_2} = \frac{-\alpha_1^2 + \alpha_1}{\alpha_1 - \alpha_1^2} = 1 
\]
\[
\sigma_3 = \frac{\alpha_1^2 - \alpha_0 \alpha_2}{\alpha_1 - \alpha_2} = 0
\]
\[
c_d = (d-1)\alpha_0 \alpha_2 - d\alpha_1^2 + \alpha_0 \alpha_1 = \alpha_1 - \alpha_1^2 = \frac{e^{-\frac{1}{\sigma^2}}}{(1 + e^{-\frac{1}{\sigma^2}})^2}
\]
And it is easy to check we also have 
\[
\begin{split}
    \sigma_0 \alpha_1 + \sigma_1\alpha_1 + (d-1)\sigma_1 \alpha_2 & = 0 \\
    \sigma_0(1-\alpha_1) + (d-1) \sigma_1(\alpha_1 - \alpha_2) = c_d \\
    \sigma_1\alpha_1 + \sigma_2 \alpha_1 + (d-1)\sigma_3\alpha_2 & = c_d \\ 
    \sigma_1\alpha_1 + \sigma_2\alpha_2 + \sigma_3 \alpha_1 + (d-2) \sigma_3 \alpha_2 & = 0 \\ 
    \sigma_1 \alpha_0 + \sigma_2 \alpha_1 + (d-1) \sigma_3\alpha_1 & = 0\\ 
    \sigma_0 \alpha_0 + d\sigma_1 \alpha_1 & = c_d \\
\end{split}
\]

Then, the bias term is 
\[
\begin{split}
    b &  = \frac{1}{c_d} \bigg[\sigma_0 \mbe[f(\*z)] + \sigma_1 \sum_{k=1}^d \mbe[z_kf(\*z)]\bigg] \\ 
    & = \frac{1}{c_d} \bigg[\sigma_0 (\mbp(z_j=1) x_i + \mbp(z_j=0)r) + \sigma_1 \mbe[z_if(\*z)] + \sum_{k=1, k
    \neq j}^d \mbe[z_kf(\*z)]\bigg] \\ 
    & = \frac{1}{c_d} \bigg[\sigma_0 (\alpha_1 x_i + (1-\alpha_1)r) + \sigma_1 \mbp(z_j=1) x_i  + \sigma_1\sum_{k=1, k
    \neq j}^d (\mbp(z_k=1, z_j = 1) x_i + \mbp(z_k=1, z_j = 0) r)\bigg] \\ 
    & =  \frac{1}{c_d} \bigg[\sigma_0 (\alpha_1 x_i + (1-\alpha_1)r) + \sigma_1 \alpha_1 x_i  + \sigma_1\sum_{k=1, k
    \neq j}^d (\alpha_2 x_i + (\alpha_1 - \alpha_2) r)\bigg] \\ 
    & = \frac{1}{c_d} \bigg[\sigma_0 (\alpha_1 x_i + (1-\alpha_1)r) + \sigma_1 \alpha_1 x_i  + (d-1) \sigma_1(\alpha_2 x_i + (\alpha_1 - \alpha_2) r)\bigg] \\ 
    & = \frac{1}{c_d}\bigg[\big(\sigma_0 \alpha_1 + \sigma_1\alpha_1 + (d-1)\sigma_1\alpha_2\big)x_i + \big(\sigma_0(1-\alpha_1) + (d-1)\sigma_1(\alpha_1 - \alpha_2)\big)r\bigg]\\ 
    & = \frac{1}{c_d}\big[0 + c_d r\big] = r \\
\end{split}
\]

For $ l\neq j$, we have 
\[
\begin{split}
    w_l & = \frac{1}{c_d} \bigg[\sigma_1 \mbe[f(\*z)] + \sigma_2 \mbe[z_l f(\*z)] + \sigma_3\sum_{k=0,k\neq l}\mbe[z_k f(\*z)] \bigg] \\ 
    & = \frac{1}{c_d}\bigg[\sigma_1 (\alpha_1 x_i + (1-\alpha_1)r) + \sigma_2(\alpha_2 x_i + (\alpha_1 - \alpha_2) r) \bigg] \\ 
    & = \frac{1}{c_d}\bigg[(\sigma_1\alpha_1 + \sigma_2 \alpha_2)x_i + (\sigma_1(1-\alpha_1) + \sigma_2(\alpha_1 - \alpha_2))r\bigg] \\ 
    & = \frac{1}{c_d}[0 + 0] = 0
\end{split}
\]

For $ l =  j$, we have 
\[
\begin{split}
    w_l & = \frac{1}{c_d} \bigg[\sigma_1 \mbe[f(\*z)] + \sigma_2 \mbe[z_l f(\*z)] + \sigma_3\sum_{k=0,k\neq l}\mbe[z_k f(\*z)] \bigg] \\ 
    & = \frac{1}{c_d}\bigg[\sigma_1 (\alpha_1 x_i + (1-\alpha_1)r) + \sigma_2\alpha_1 x_i\bigg] \\ 
    & = \frac{1}{c_d}\bigg[(\sigma_1\alpha_1 + \sigma_2 \alpha_1)x_i + \sigma_1(1-\alpha_1)r\bigg] \\ 
    & = \frac{1}{c_d}[c_d x_i - c_d r] = x_i - r
\end{split}
\]
Therefore, for $f(\*x) = x_i$ and $x_i$ in superpixel $j$, we have 
\[
w_j = x_i - r, w_k = 0, \forall k \neq j, b = r
\]

For more general $f(\*x) = \sum_i c_i x_i = \sum_i c_i f_i(\*x), f_i(\*x) = x_i$, we have 
\[
\begin{split}
    b & = \frac{1}{c_d} \bigg[\sigma_0 \mbe[f(\*z)] + \sigma_1 \sum_{k=1}^d \mbe[z_kf(\*z)]\bigg] =   \frac{1}{c_d} \bigg[\sigma_0 \mbe[\sum_i c_i f_i(\*z)] + \sigma_1 \sum_{k=1}^d \mbe[z_k c_i f_i(\*z)]\bigg] \\
    & =  \sum_i c_i \frac{1}{c_d} \bigg[\sigma_0 \mbe[f_i(\*z)] + \sigma_1 \sum_{k=1}^d \mbe[z_k\sum_i f_i(\*z)]\bigg] \\
    & = \sum_i c_i r_i 
\end{split}
\]
where $r_i$ is the baseline value set for pixel $i$. 
We also have 
\[
\begin{split}
    w_l & = \frac{1}{c_d} \bigg[\sigma_1 \mbe[f(\*z)] + \sigma_2 \mbe[z_l f(\*z)] + \sigma_3\sum_{k=0,k\neq l}\mbe[z_k f(\*z)] \bigg] \\ 
    & = \frac{1}{c_d} \bigg[\sigma_1 \mbe[ \sum_i c_i f_i(\*z) ] + \sigma_2 \mbe[z_l  \sum_i c_i f_i(\*z) ] \bigg] \\ 
    & =\sum_i c_i \frac{1}{c_d} \bigg[\sigma_1 \mbe[  f_i(\*z) ] + \sigma_2 \mbe[z_l f_i(\*z) ] \bigg] \\ 
    & = \sum_i c_i \frac{1}{c_d} \bigg[\sigma_1 \mbe[  f_i(\*z) ] + \sigma_2 \mbe[z_l f_i(\*z) ] \bigg] \\ 
    & =  \sum_{i\notin \text{ superpixel } l} c_i \frac{1}{c_d} \bigg[\sigma_1 \mbe[  f_i(\*z) ] + \sigma_2 \mbe[z_l f_i(\*z) ] \bigg] +  \sum_{i\in \text{ superpixel } l} c_i \frac{1}{c_d} \bigg[\sigma_1 \mbe[  f_i(\*z) ] + \sigma_2 \mbe[z_l f_i(\*z) ] \bigg] \\ 
    & = \sum_{i\in \text{ superpixel } l} c_i ( x_i - r_i ) \\ 
\end{split}
\]

\section{Exact Expression for Gaussian Distribution: Linear Case}
\subsection{Exact Expression of $\Sigma$}
$z_i \sim \mathcal{N}(\mathbf{1}, \sigma^2\*I), \forall i=1,\cdots, d$. In this case 
\[
\hat{\Sigma}_n = \begin{bmatrix}
    \frac{1}{n}\sum_k 1& \frac{1}{n}\sum_k z_{k1} & \cdots & \frac{1}{n}\sum_k z_{kd} \\ 
    \frac{1}{n}\sum_k z_{k1} & \frac{1}{n} \sum_k z_{k1}^2 & \cdots & \frac{1}{n}\sum_k z_{l1}z_{kd} \\ 
    \vdots & \vdots & \ddots & \vdots \\ 
     \frac{1}{n}\sum_k z_{k1} &  \frac{1}{n}\sum_k z_{kd} z_{k1} & \cdots &  \frac{1}{n}\sum_k z_{kd}^2\\
\end{bmatrix}
\]
Then we have 
\[
\Sigma = \begin{bmatrix}
    1 & 1 & \cdots & 1 \\ 
    1 & 1 + \sigma^2 & \cdots & 1 \\ 
    \vdots & \vdots & \ddots & \vdots \\ 
    1 & 1 & \cdots & 1 + \sigma^2 \\ 
\end{bmatrix}
\]
\[
\Sigma^{-1} = \begin{bmatrix}
    1 + \frac{d}{\sigma^2}& -\frac{1}{\sigma^2} & \cdots & -\frac{1}{\sigma^2} \\ 
    -\frac{1}{\sigma^2} & \frac{1}{\sigma^2} & \cdots & 0 \\ 
    \vdots & \vdots & \ddots & \vdots \\ 
    -\frac{1}{\sigma^2} & 0 & \cdots & \frac{1}{\sigma^2} \\ 
\end{bmatrix}
\]
For linear model $f(\*x) = x_i $, we have 
\[
\mathbb{E}[f(\*z)] = x_i, \mbe[z_jf(\*z)] = \mbe[z_j^2 x_i] = (1 + \sigma^2 ) x_i, \mbe[z_lf(\*z)] = \mbe_{z_l}[z_l]\mbe_{\*z}[f(\*z)] = x_i 
\]
Then, we have 
\[
b = \Sigma^{-1}_{1,\cdot} \Gamma = (1+\frac{d}{\sigma^2})\mathbb{E}[f(\*z)] - \frac{1}{\sigma^2}\sum_l \mbe[z_lf(\*z)] = (1+\frac{d}{\sigma^2})x_i - \frac{(d-1)}{\sigma^2} x_i - \frac{1 + \sigma^2}{\sigma^2}x_i = 0
\]
\[
w_j = -\frac{1}{\sigma^2}\mathbb{E}[f(\*z)] + \frac{1}{\sigma^2}  \mbe[z_jf(\*z)] = -\frac{1}{\sigma^2}x_i + \frac{1}{\sigma^2}(1 + \sigma^2) x_i = x_i 
\]
\[
w_l = -\frac{1}{\sigma^2}\mathbb{E}[f(\*z)] + \frac{1}{\sigma^2}  \mbe[z_lf(\*z)] = -\frac{1}{\sigma^2}x_i + \frac{1}{\sigma^2}x_i = 0, \forall l \neq j 
\]
By linearity, we have for more general linear models $f(\*x) = \sum_i c_i x_i $, we have 
\[
b = 0, w_j = \sum_{i \in \text{ superpixel } j}c_i x_i 
\]
\end{proof}
